# Supplementary material for: Tensor Normal Training for Deep Learning Models
Source: arXiv:2106.02925 source file (2021-12-21)
Supplement: Supplementary file 1 [file damping.tex]

\subsection{}

We first focus on the case of order-2 tensor. Let $G \in R^{m \times n}$ denotes a random matrix. 
% Following the Definition 2.2.1 in \cite{gupta2018matrix}, 
We {assume} that $G$ follows a \textbf{matrix normal} distribution
{(see e.g. \cite{dees2019statistically})}
with mean zero and covariance matrix $V \otimes U$, where $V \in R^{m \times m}$ and $U \in R^{n \times n}$. By the definition, $\overline{\text{vec}}(G) \sim Normal(0, V \otimes U)$, where $\overline{\text{vec}}$ denotes row-major vectorization.

We define the variance of $G$ as $var(G) := \E \left[ ||G - \E[G]||^2 \right]$. Immediately, we have that
\begin{align}
    var(G)
    % := \E \left[ ||G - \E[G]||^2 \right]
    = \E \left[ ||G||^2 \right]
    = \E \left[ ||\overline{\text{vec}}(G)||^2 \right]
    = \E \left[ \text{tr} \left( \overline{\text{vec}}(G) \overline{\text{vec}}(G)^\top \right) \right]
    = \text{tr} \left( cov \left( \overline{\text{vec}}(G) \right) \right)
    = \text{tr} \left( V \otimes U \right).
    \label{eq_3}
\end{align}

Another useful property can be derived from {(24) in \cite{dees2019statistically}}:
\begin{align}
    \mathbb{E} (G G^\top) = V \cdot \text{tr}(U)
    \label{eq_4}
    \\
    \mathbb{E} (G^\top G) = U \cdot \text{tr}(V)
    \label{eq_5}
\end{align}

Note that a matrix normal distribution can have multiple sets of parameters $(U, V)$, because $c U \otimes \frac{1}{c} V = U \otimes V$ for $c > 0$. 
Moreover, we can actually rewrite the covariance to be
{$c (c_U \mathbb{E} (G^\top G)) \otimes (c_V \mathbb{E} (G G^\top)) := c \cdot \tilde{U} \otimes \tilde{V}$}.
The choice of $c_U$, $c_V$ is important because when damping is involved, the inverse covarance is approximated by 
{$c^{-1} (\tilde{U} + \epsilon I)^{-1} \otimes (\tilde{V} + \epsilon I)^{-1}$}.

Following we introduce several ways of estimating $U$ and $V$, which leads to optimization methods with $V^{-1} \otimes U^{-1}$ as the preconditioning matrix.

Following we discuss various choices of $c_U$, $c_V$, and $c$: 

\begin{itemize}
    \item We impose {$c = 1$}: 
    \begin{itemize}
        \item We further impose that $\text{tr}(\tilde{U}) = \text{tr}(\tilde{V})$: 
        \clarify{haven't try yet}
        
        We have that
        \begin{align}
            \tilde{U} = \frac{\mathbb{E} (G^\top G)}{\sqrt{\text{tr}(\mathbb{E} (G^\top G))}}, \tilde{V} = \frac{\mathbb{E} (G G^\top)}{\sqrt{\text{tr}(\mathbb{E} (G^\top G))}}.
            \label{eq_7}
        \end{align}
        
    \addthis{Note that $\text{tr}(\mathbb{E} (G^\top G)) = \text{tr}(\mathbb{E} (G G^\top))$.}
        
    %   \clarify{Shouldn't the denominator in the definition of
    %   $\tilde V$ be 
    %   $\sqrt{\text{tr}(\mathbb{E} (G G^\top ))}$?}
        
        \item

        Let $d_U$, $d_V$ denote the dimension of $U$, $V$, respectively.
        Hence, we {impose} that $\frac{\text{tr}(\tilde{U})}{d_U} = \frac{\text{tr}(\tilde{V})}{d_V}$, which can be viewed as requiring the average eigenvalues of $\tilde{U}$ and $\tilde{V}$ to be the same. By (\ref{eq_4}) and (\ref{eq_5}), we can get the expression of $\tilde{U}$ and $\tilde{V}$:
    
        $$c_U = \sqrt{\frac{d_U}{d_V \text{tr}( \mathbb{E} (G G^\top))}},
        \quad
        c_V = \sqrt{\frac{d_V}{d_U \text{tr}( \mathbb{E} (G G^\top))}}$$

        \clarify{this is matrix-normal-same-trace}
    \end{itemize}

    \item We do NOT impose
    % \deletethis{$c_U c_V$ = 1}
    {$c = 1$}: 
    \begin{itemize}
        \item 
        We impose $\text{tr}(\tilde{U}) = \text{tr}(\tilde{V}) = 1$, which is essentially what \cite{dees2019statistically} proposed.

    %     \addthis{
    % \cite{dees2019statistically}:
    
    % To resolve this so-called "non-identifiability" issue, we re-parameterize matrix-normal distribution with $\sigma^2$, $\tilde{U}$ and $\tilde{V}$, where
    % \begin{align*}
    %     & V \otimes U = \sigma^2 \left( \tilde{V} \otimes \tilde{U} \right)
    %     \\
    %     & \text{tr}(\tilde{U}) = \text{tr}(\tilde{V}) = 1
    % \end{align*}
    
    % By (\ref{eq_3}), 
    % \begin{align*}
    %     var(G)
    %     = \text{tr} \left( \sigma^2 \left( \tilde{V} \otimes \tilde{U} \right) \right)
    %     = \sigma^2 \text{tr} \left( \tilde{V} \otimes \tilde{U} \right)
    %     = \sigma^2 \text{tr} ( \tilde{V} ) \text{tr} ( \tilde{U} )
    %     = \sigma^2.
    % \end{align*}
    % Hence, we can estimate $\sigma^2$ by $var(G)$. Moreover, by (\ref{eq_4}) and (\ref{eq_5}) we have that
    % \begin{align*}
    %     & \E (G G^\top)
    %     = V \cdot \text{tr}(U)
    %     = \frac{V}{\text{tr}(V)} \cdot \text{tr}(V) \cdot \text{tr}(U)
    %     = \tilde{V} \cdot \sigma^2
    % \\
    %     & \E (G^\top G) = \tilde{U} \cdot \sigma^2
    % \end{align*}
    % Hence, we can estimate $\tilde{U}$, $\tilde{V}$ by $\frac{1}{\sigma^2} \E (G^\top G)$,  $\frac{1}{\sigma^2} \E (G G^\top)$, respectively. 
    
    % }
    
        \clarify{haven't done yet}

        \item 
        
        We impose $\tilde{V} = \mathbb{E} (G G^\top)$,
        $\tilde{U} = \mathbb{E} (G^\top G)$, which is similar as in Shampoo.
        
        Recall that the covariance is
        % \deletethis{$\frac{1}{c_U c_V} \tilde{U} \otimes \tilde{V}$}
        {$c \tilde{U} \otimes \tilde{V}$} where $\tilde{V} = \mathbb{E} (G G^\top)$, $\tilde{U} = \mathbb{E} (G^\top G)$. Thus, 
        % \deletethis{$c_U c_V = \text{tr}(U) \text{tr}(V) = \text{tr}(\mathbb{E} (G G^\top))$}
        {$c = \text{tr}(U) \text{tr}(V) = \text{tr}(\mathbb{E} (G G^\top))$}.
    
        Note that in Shampoo, we do SVD on $L + \epsilon I$ and $R + \epsilon I$, where $L \approx \mathbb{E} (G G^\top)$, $R \approx \mathbb{E} (G^\top G)$.

    \clarify{this is matrix-normal in the legend}
        
    %     \addthis{
    %     Hence, the inverse of the co-variance matrix of $\overline{\text{vec}}(G)$ is
    % \begin{align*}
    %     (V \otimes U)^{-1}
    %     & = V^{-1} \otimes U^{-1}
    %     = \left( \frac{\mathbb{E} (G G^\top)}{\text{tr}(V)} \right)^{-1} \otimes \left( \frac{\mathbb{E} (G^\top G)}{\text{tr}(U)} \right)^{-1}
    %     \\
    %     & = \text{tr}(U) \text{tr}(V) \left( \mathbb{E} (G G^\top)^{-1} \otimes \mathbb{E} (G^\top G) \right)^{-1}
    % \end{align*}
    % where
    % \begin{align*}
    %     \text{tr}(U) \text{tr}(V) = \mathbb{E} (\text{tr} (G G^\top)) 
    % \end{align*}
    % }
    
    %     \addthis{
    %     If we interpret Shampoo under the "matrix normal" model, we know that 
    % \begin{align*}
    %     L \approx \mathbb{E} (G G^\top)
    %     \\
    %     R \approx \mathbb{E} (G^\top G)
    % \end{align*}
    % Hence, the way Shampoo approximates the inverse of co-variance matrix (i.e. $V^{-1} \otimes U^{-1}$) is by
    % \begin{align*}
    %     L^{-1/2} \otimes R^{-1/2} = (\mathbb{E} (G G^\top))^{-1/2} \otimes (\mathbb{E} (G^\top G))^{-1/2}
    % \end{align*}
    
    % % When Shampoo performs the inversion (or SVD) of $L$ and $R$, it is actually on $L + \epsilon I$ and $R + \epsilon I$. 
    % }

    \end{itemize}
\end{itemize}

\subsection{}

Note that in Shampoo, the empirical Fisher is approximated by
\begin{align*}
    ((H^1 + \epsilon I) \otimes \cdots \otimes (H^k + \epsilon I))^{1/k}
\end{align*}
Hence, the total "magnitude" of damping is approximately $\epsilon$ (to the power of 1). On the other hand, we also want $\mathbb{E} [G^{(i)}] + \epsilon^{(i)} I$ to share the same trace, because $\mathbb{E} [G^{(i)}]$ shares the same trace in the first place.
