# Supplementary material for: Tensor Normal Training for Deep Learning Models
Source: arXiv:2106.02925 source file (2021-12-21)
Supplement: Supplementary file 2 [file experiment_not_used.tex]

\subsection{Fashion-MNIST}

\begin{table}[H]
    \centering
    \begin{tabular}{c|c|c|c|c|c}
        Layer name & Filter/window & Input size & Output size & Input channel & Output channel \\
         \hline
        conv & $5 \times 5$ & $28 \times 28$ & $28 \times 28$ & 1 & 32
        \\
        \hline
        max pool & $2 \times 2$ & $28 \times 28$ & $14 \times 14$
        \\
        \hline
        conv & $5 \times 5$ & $14 \times 14$ & $14 \times 14$ & 32 & 64
        \\
        \hline
        max pool & $2 \times 2$ & $14 \times 14$ & $7 \times 7$
        \\
        \hline
        fully-connected & & $7 \times 7 \times 64 = 3136$ & 1024
        \\
        \hline 
        fully-connected & & 1024 & 10
        \\
        \hline
    \end{tabular}
    \caption{Architecture for Fashion-MNIST (see \cite{choi2019empirical})}
\end{table}

% Simple CNN is identical to the base model described in Shallue et al. (2019). 
% It consists of 2 convolutional layers with max pooling followed by 1 fully connected layer. 
% The convolutional layers use 5 × 5 filters with stride 1, “same” padding, and ReLU activation function. 
% Max pooling uses a 2 × 2 window with stride 2. 
% Convolutional layers have 32 and 64 filters each and the fully connected layer has 1024 units. 
% It does not use batch normalization.

\begin{table}[H]
    \centering
    \begin{tabular}{c|c|c|c|c|c}
        Layer name & Filter/window & Input size & Output size & Input channel & Output channel \\
         \hline
        conv & $5 \times 5$ & $28 \times 28$ & $28 \times 28$ & 1 & 32
        \\
        \hline
        max pool & $2 \times 2$ & $28 \times 28$ & $14 \times 14$
        \\
        \hline
        conv & $5 \times 5$ & $14 \times 14$ & $14 \times 14$ & 32 & 64
        \\
        \hline
        GAP & & $14 \times 14$ & 1
        \\
        \hline
        fully-connected & & 64 & 1024
        \\
        \hline 
        fully-connected & & 1024 & 10
        \\
        \hline
    \end{tabular}
    \caption{Architecture for Fashion-MNIST with global average pooling (GAP)}
\end{table}

\subsection{SOTA}

CIFAR10 + VGG16: 92.63\%\footnote{\url{https://github.com/chengyangfu/pytorch-vgg-cifar10}}

CIFAR10 + VGG16BN: 92.64\%\footnote{\url{https://github.com/kuangliu/pytorch-cifar}}, 93.56\%\footnote{\url{https://github.com/geifmany/cifar-vgg}}, 93.86\%\footnote{\url{https://github.com/chengyangfu/pytorch-vgg-cifar10}}

CIFAR10 + ResNet32: 92.63\%\footnote{\url{https://github.com/akamaster/pytorch_resnet_cifar10}}, 92.64\%\footnote{\url{https://github.com/junyuseu/pytorch-cifar-models}}

CIFAR100 + VGG16BN: 72.93\%\footnote{\url{https://github.com/weiaicunzai/pytorch-cifar100}}, 70.48\%\footnote{\url{https://github.com/geifmany/cifar-vgg}}

\subsection{SOTA Results}

\begin{figure}[H]
    \centering
    \includegraphics[width=\textwidth]{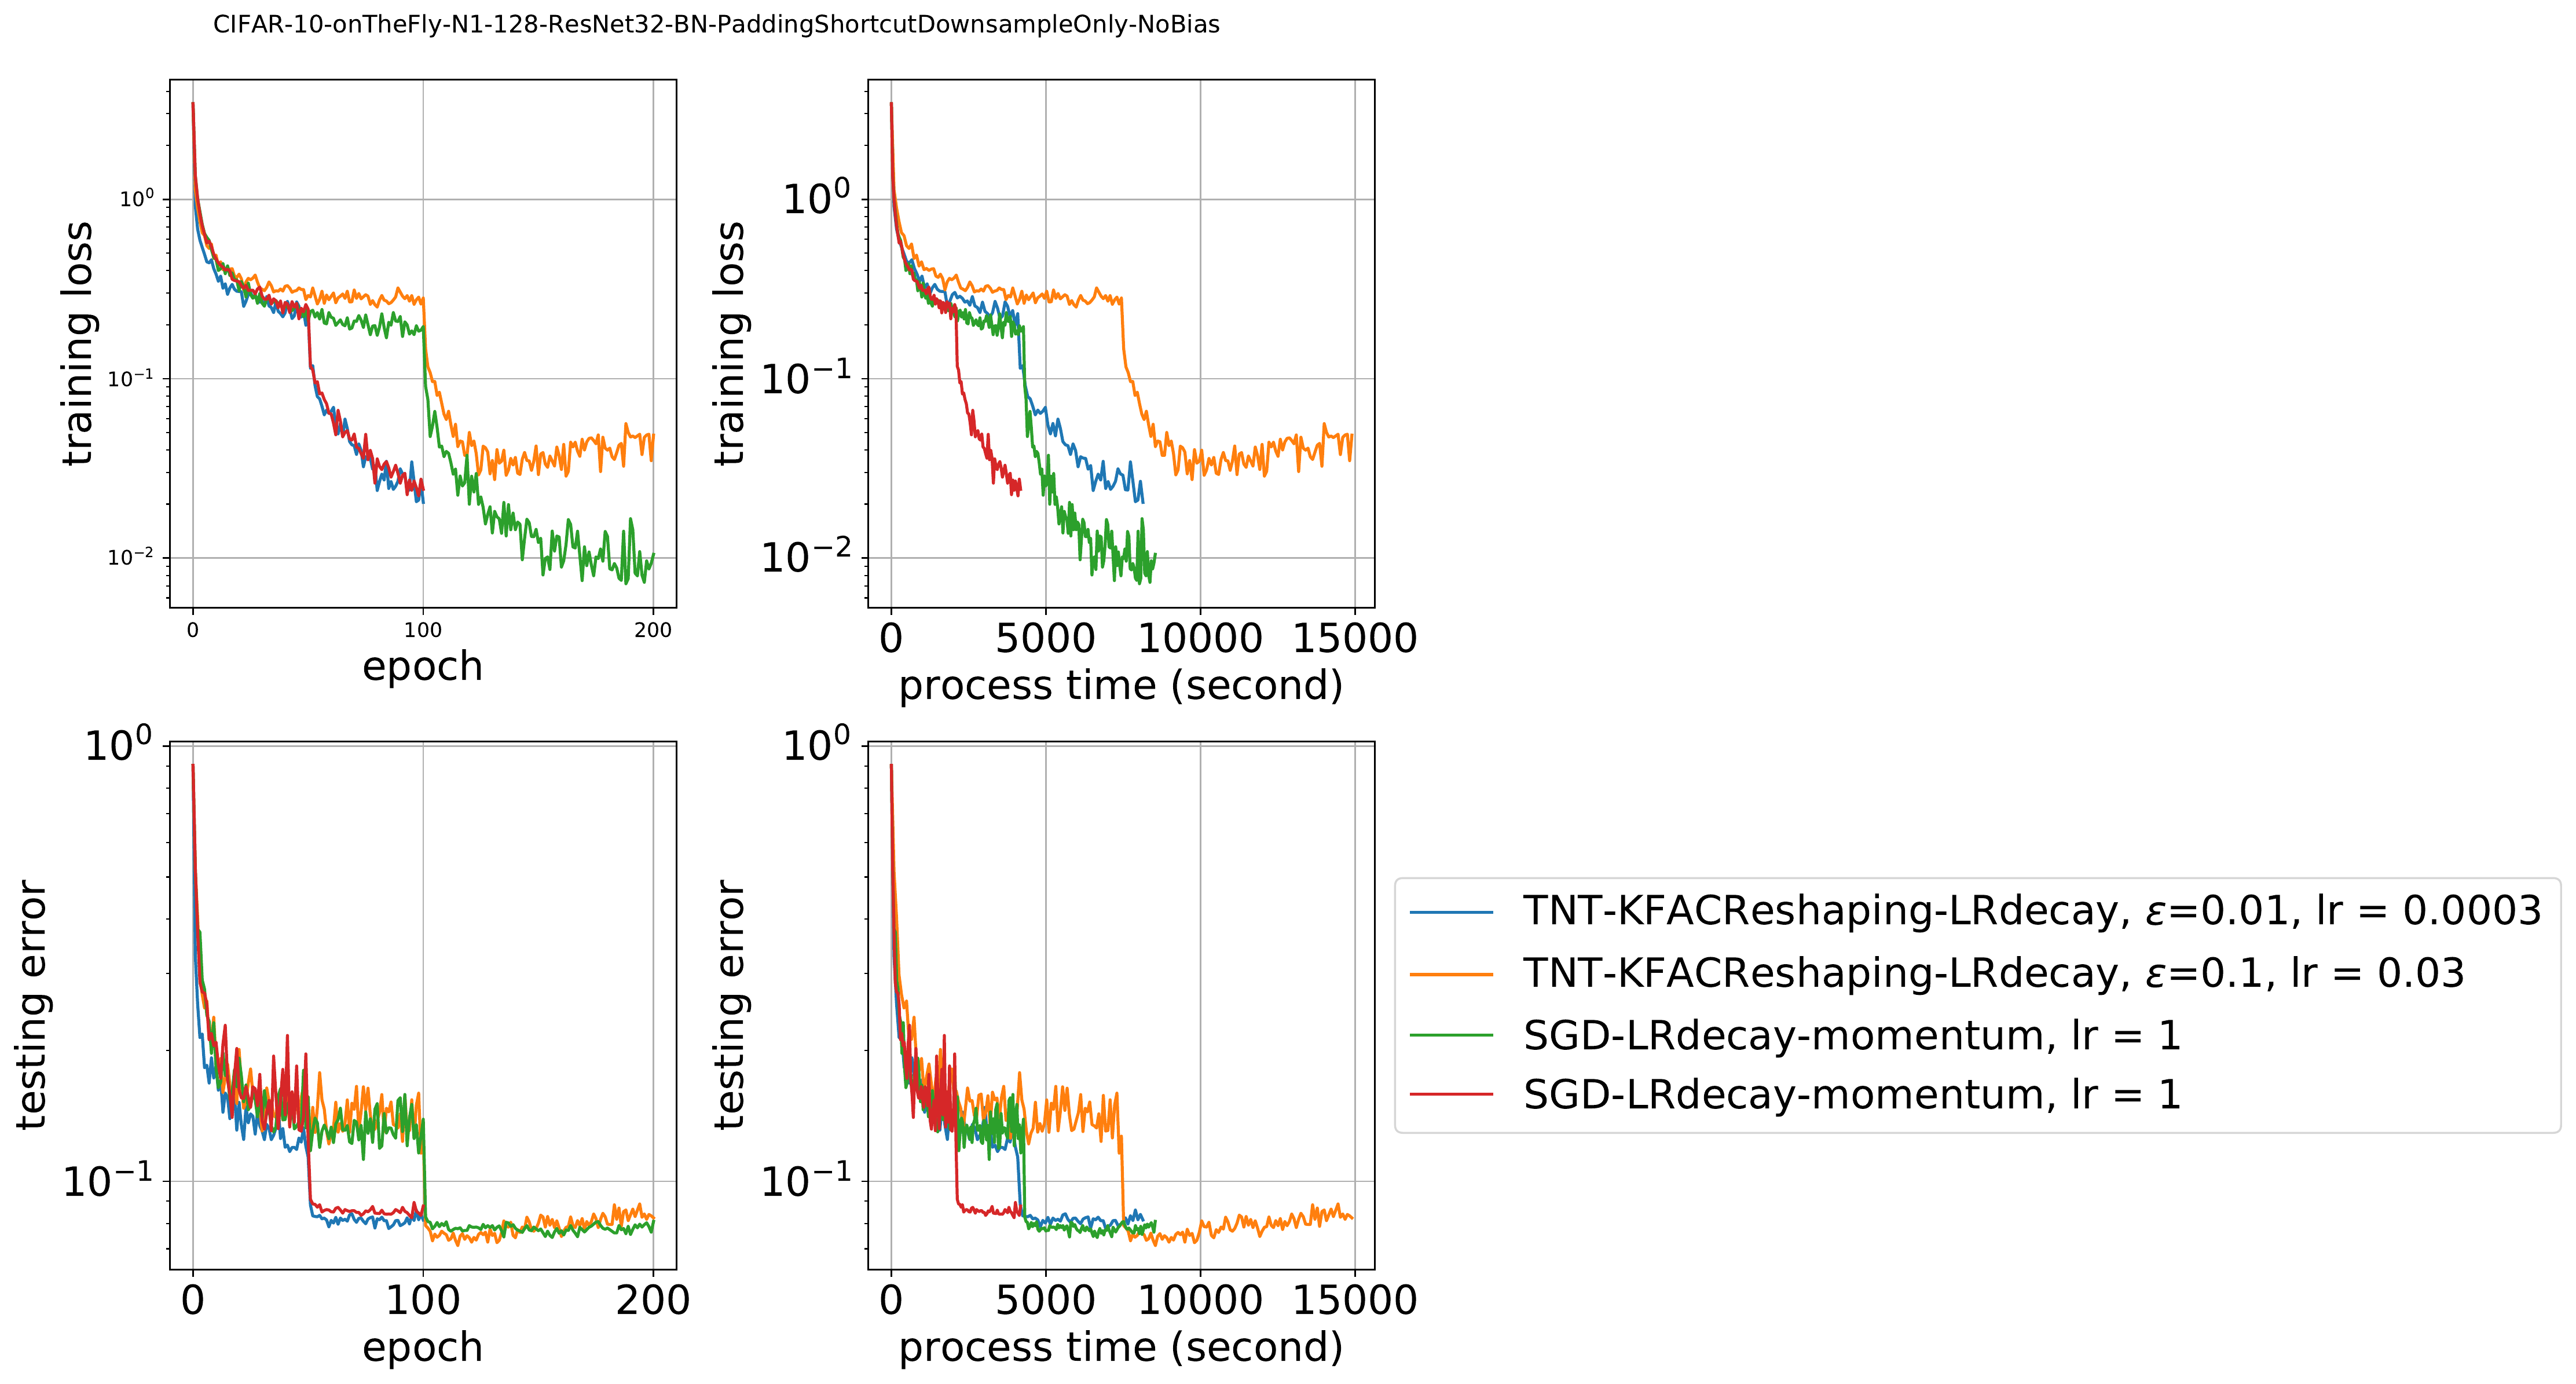}
    \caption{CIFAR-10, ResNet32}
\end{figure}

\subsection{Same Time Results}

\begin{figure}[H]
    \centering
    \includegraphics[width=\textwidth]{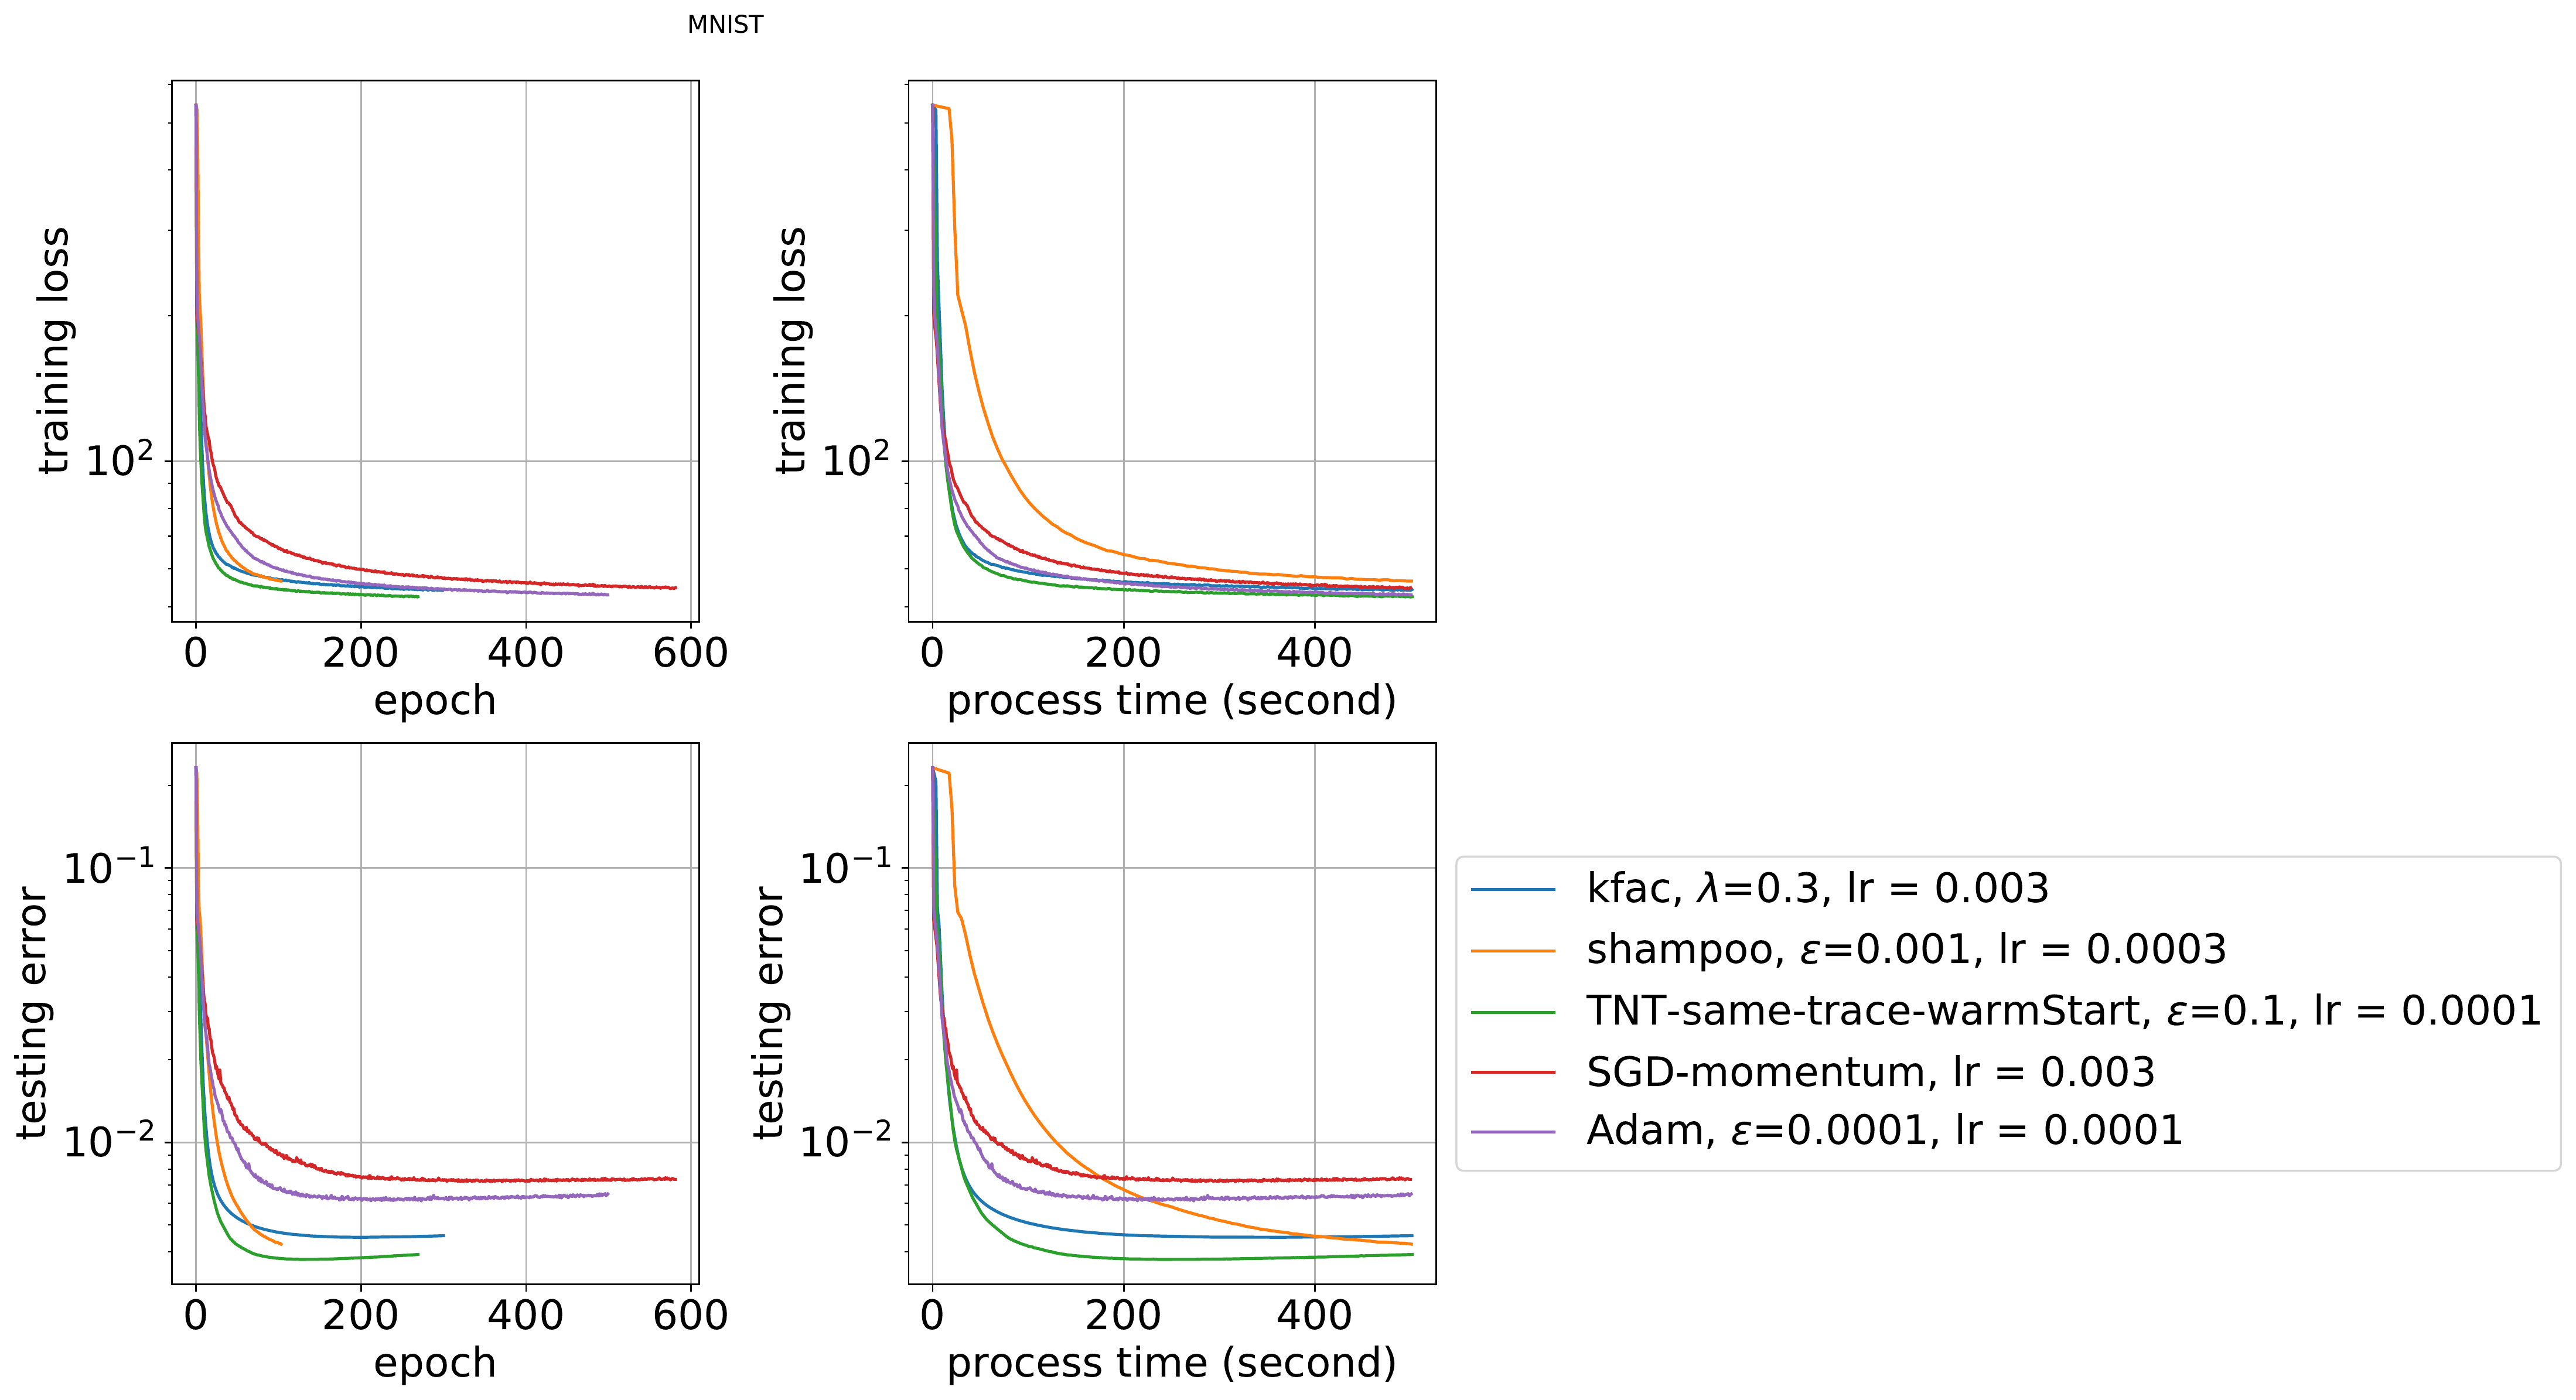}
    \caption{MNIST autoencoder}
\end{figure}

\begin{figure}[H]
    \centering
    \includegraphics[width=\textwidth]{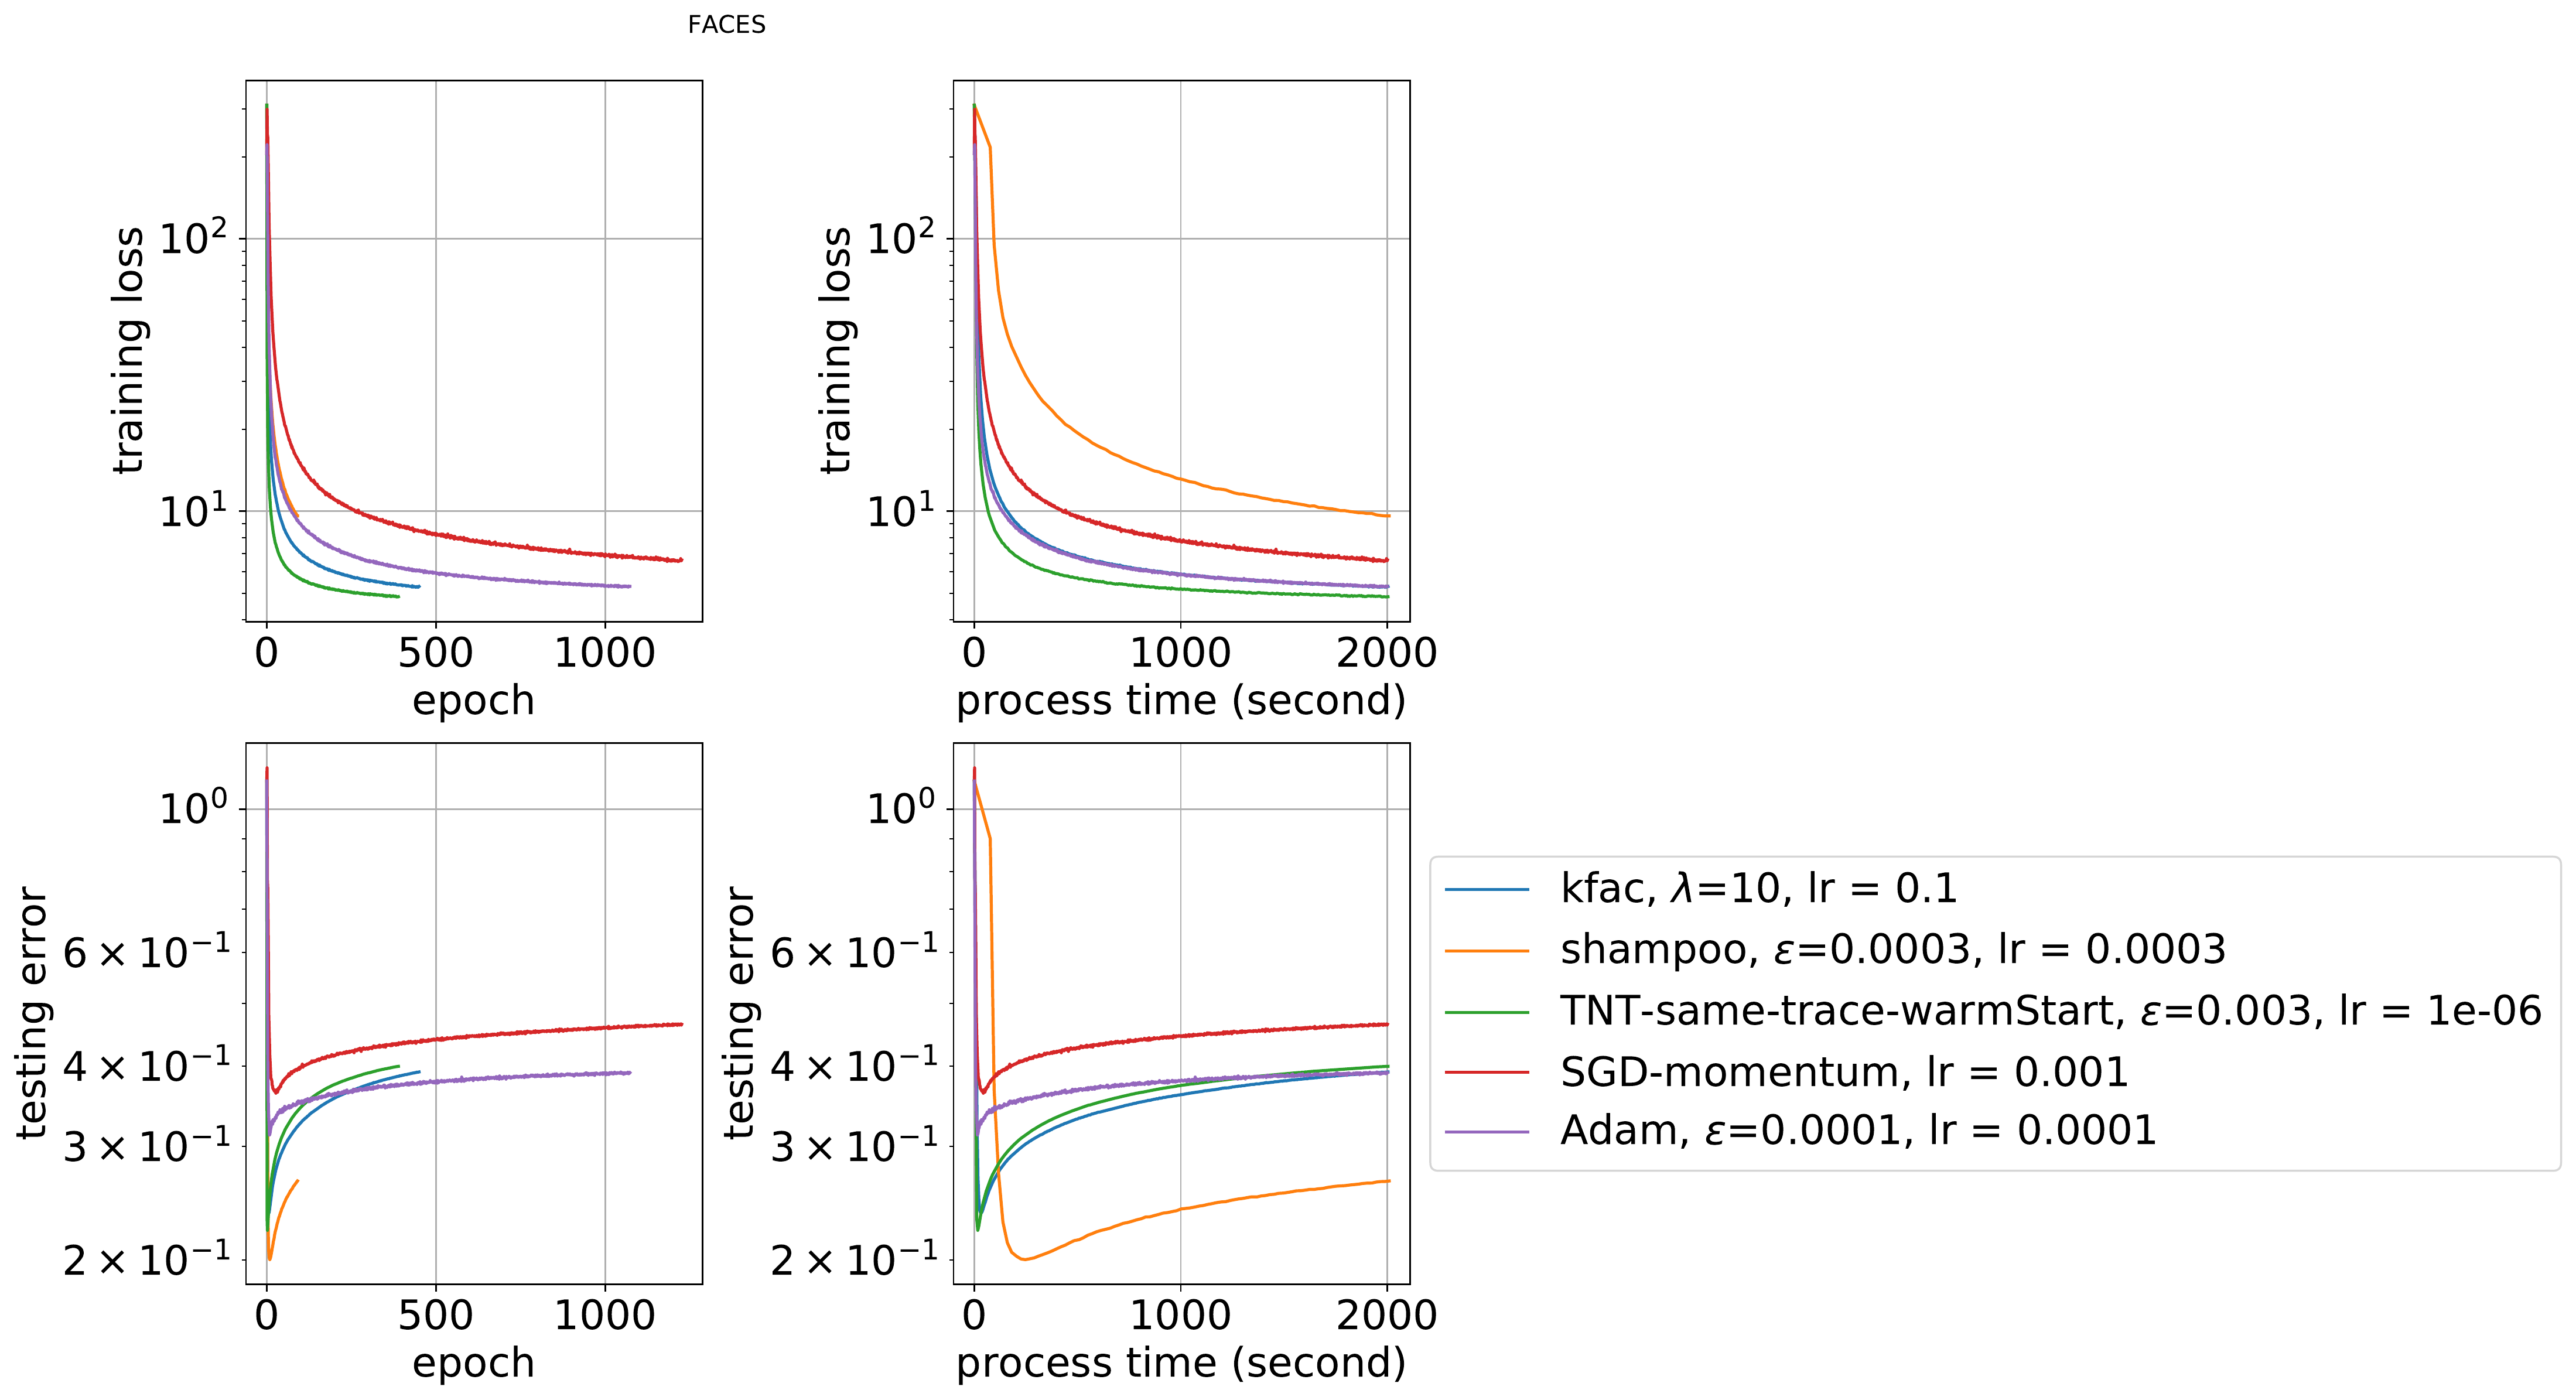}
    \caption{FACES autoencoder}
\end{figure}

\subsection{(same epochs) Results}

\begin{figure}[H]
    \centering
    \includegraphics[width=\textwidth]{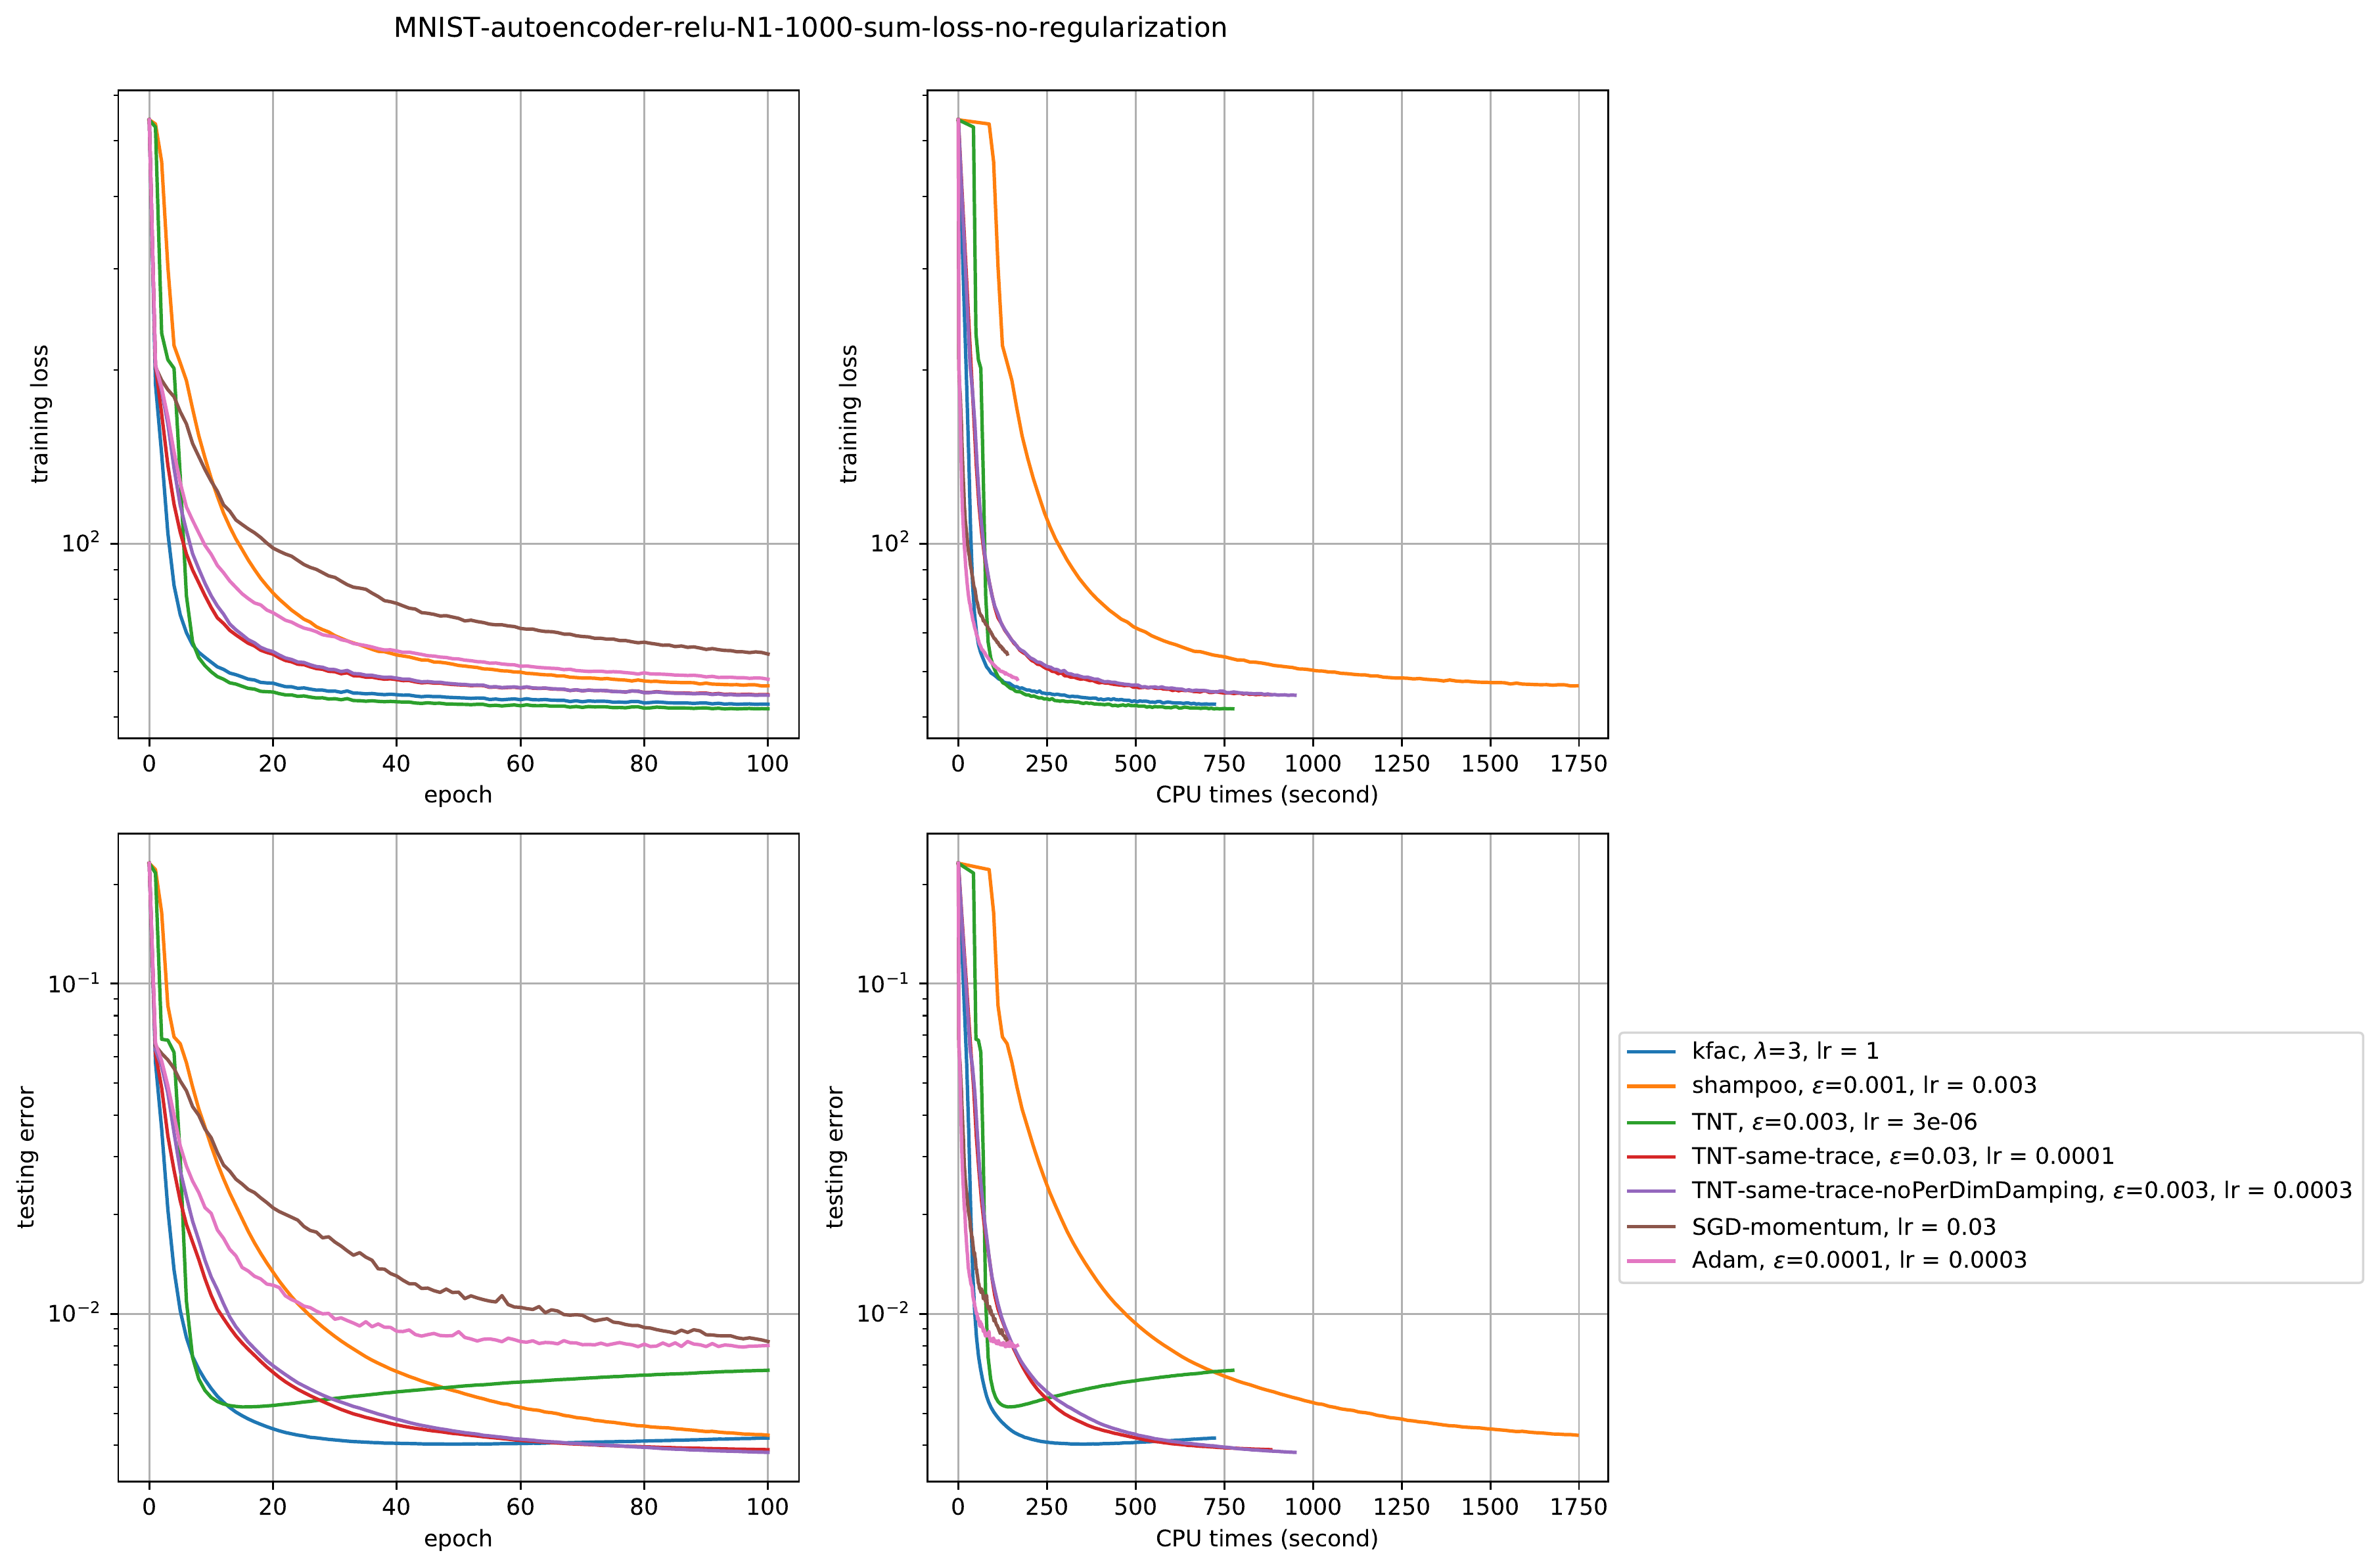}
    \caption{MNIST autoencoder}
\end{figure}

\begin{figure}[H]
    \centering
    \includegraphics[width=\textwidth]{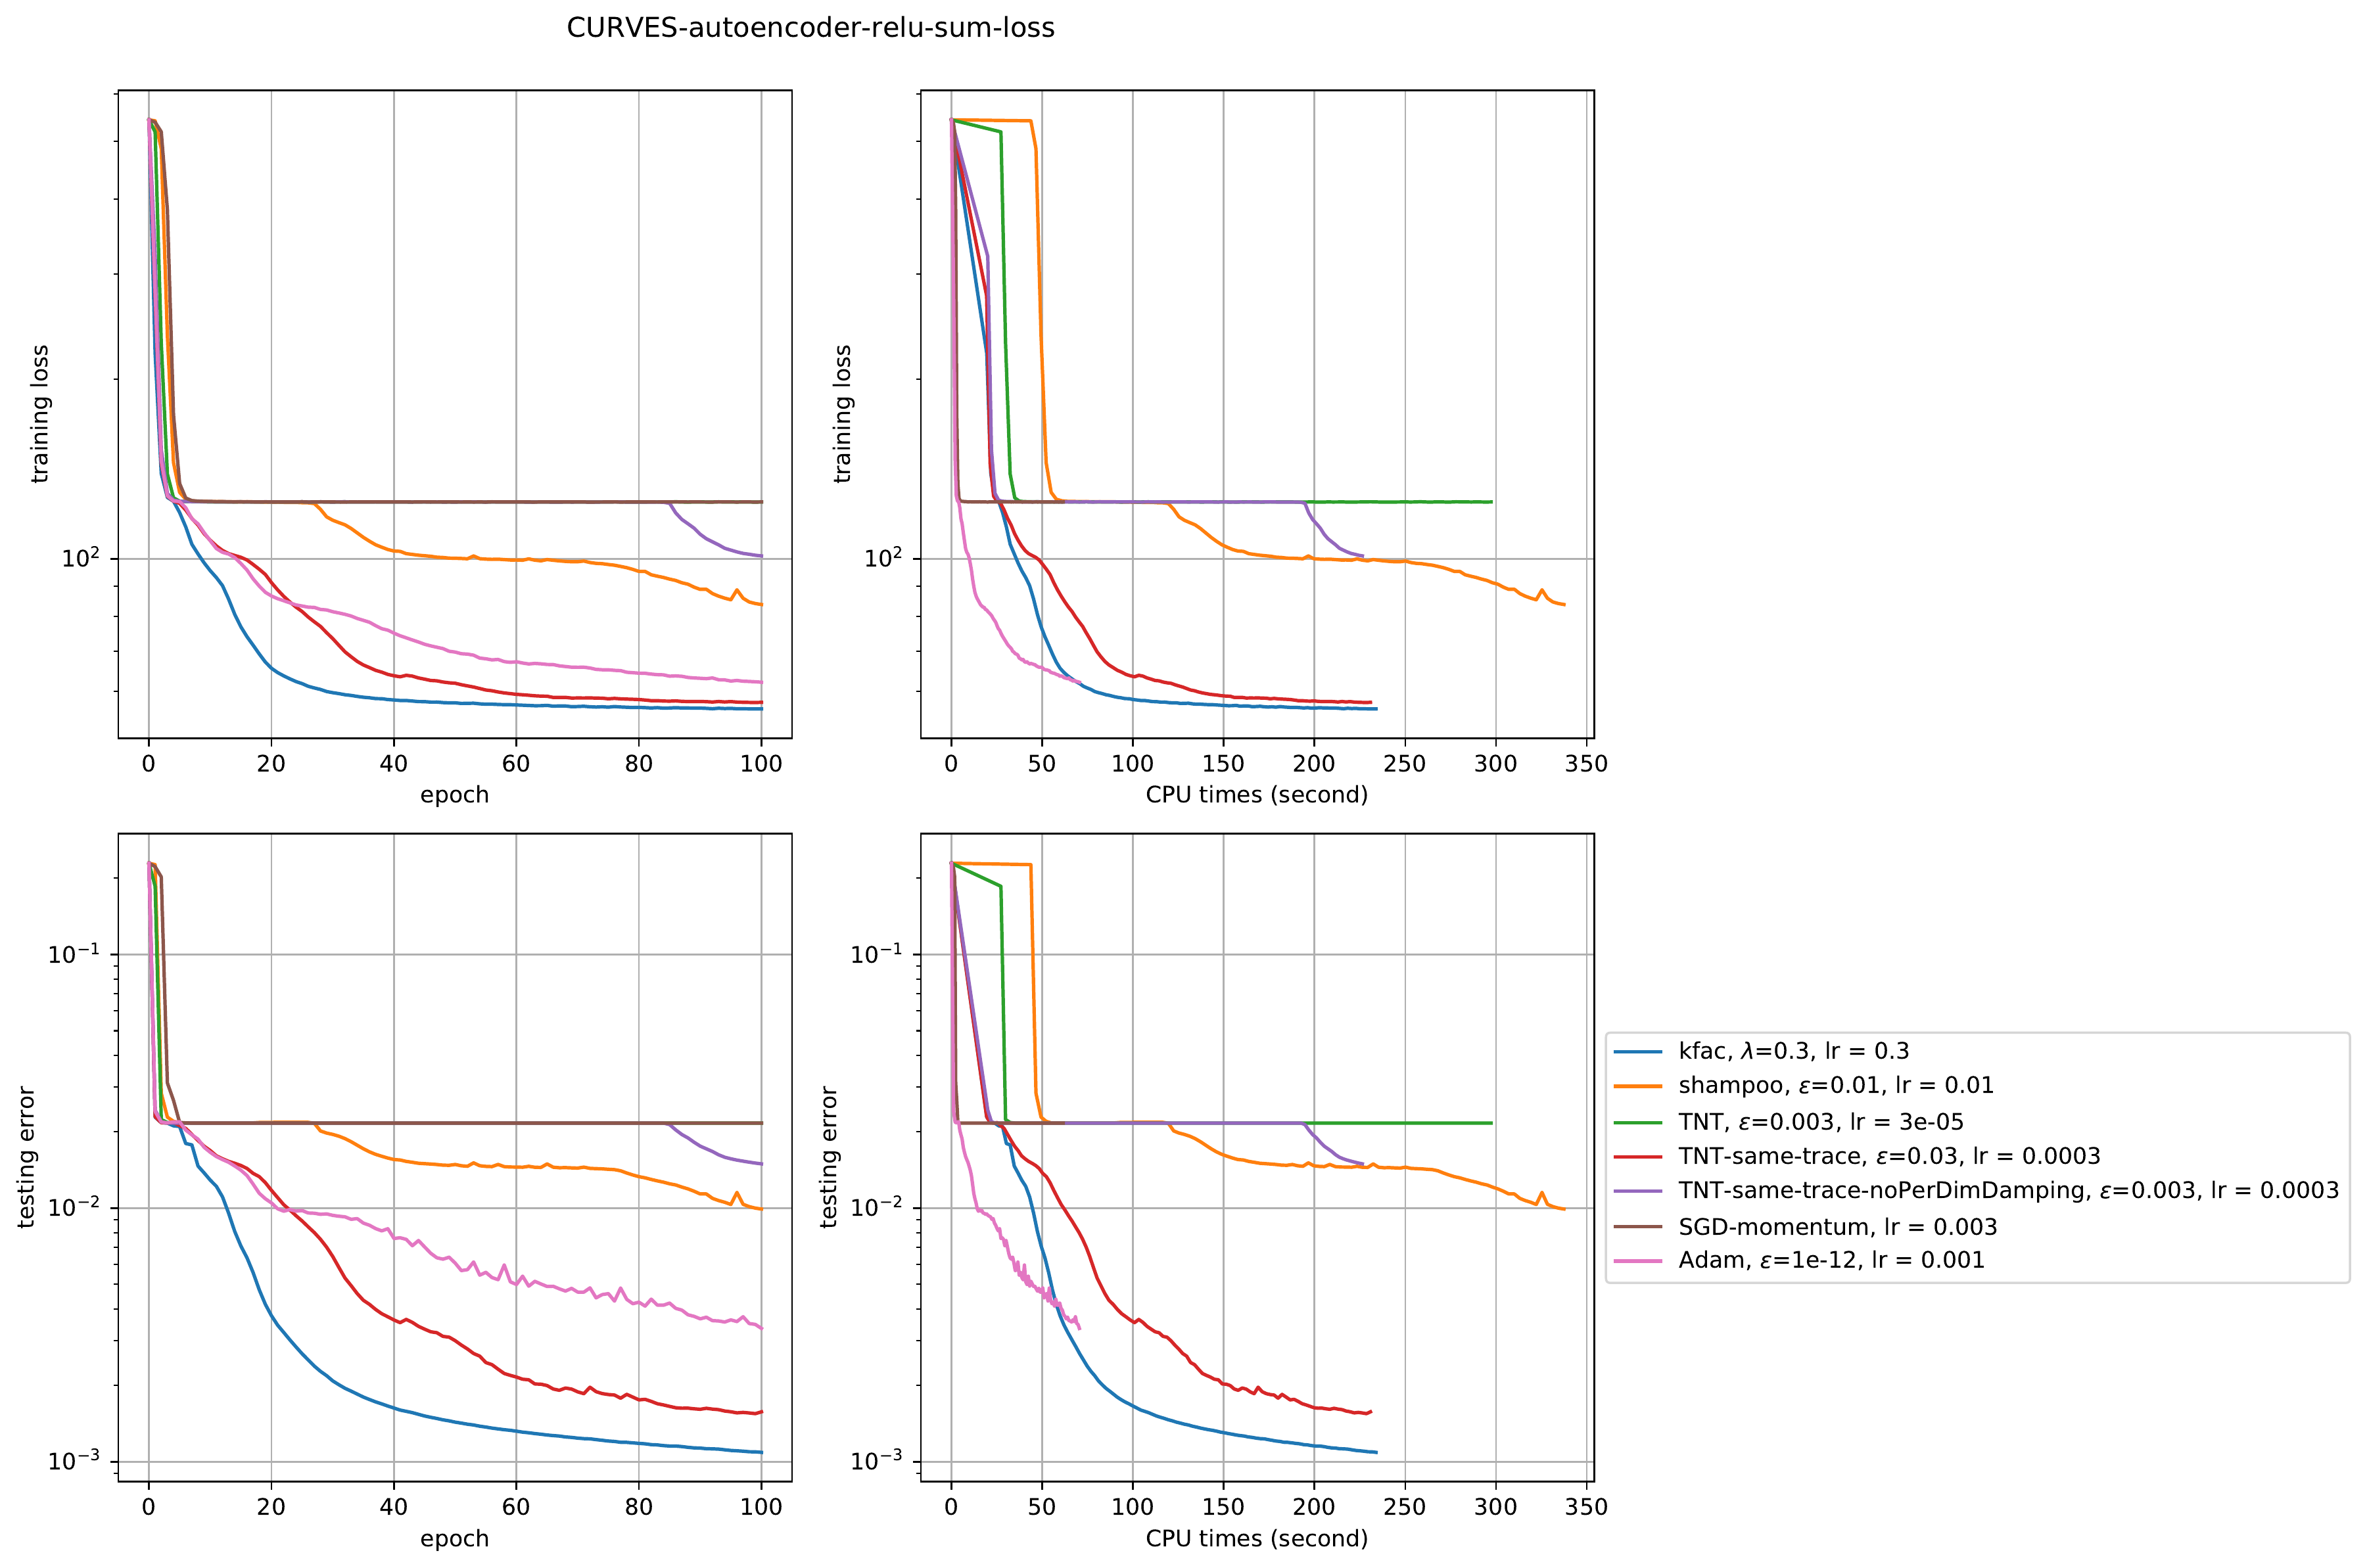}
    \caption{CURVES autoencoder}
\end{figure}

Fig
\ref{fig_2}, \ref{fig_5}, \ref{fig_4},
\ref{fig_6},
\ref{fig_7}.

\begin{figure}[H]
    \centering
    \includegraphics[width=\textwidth]{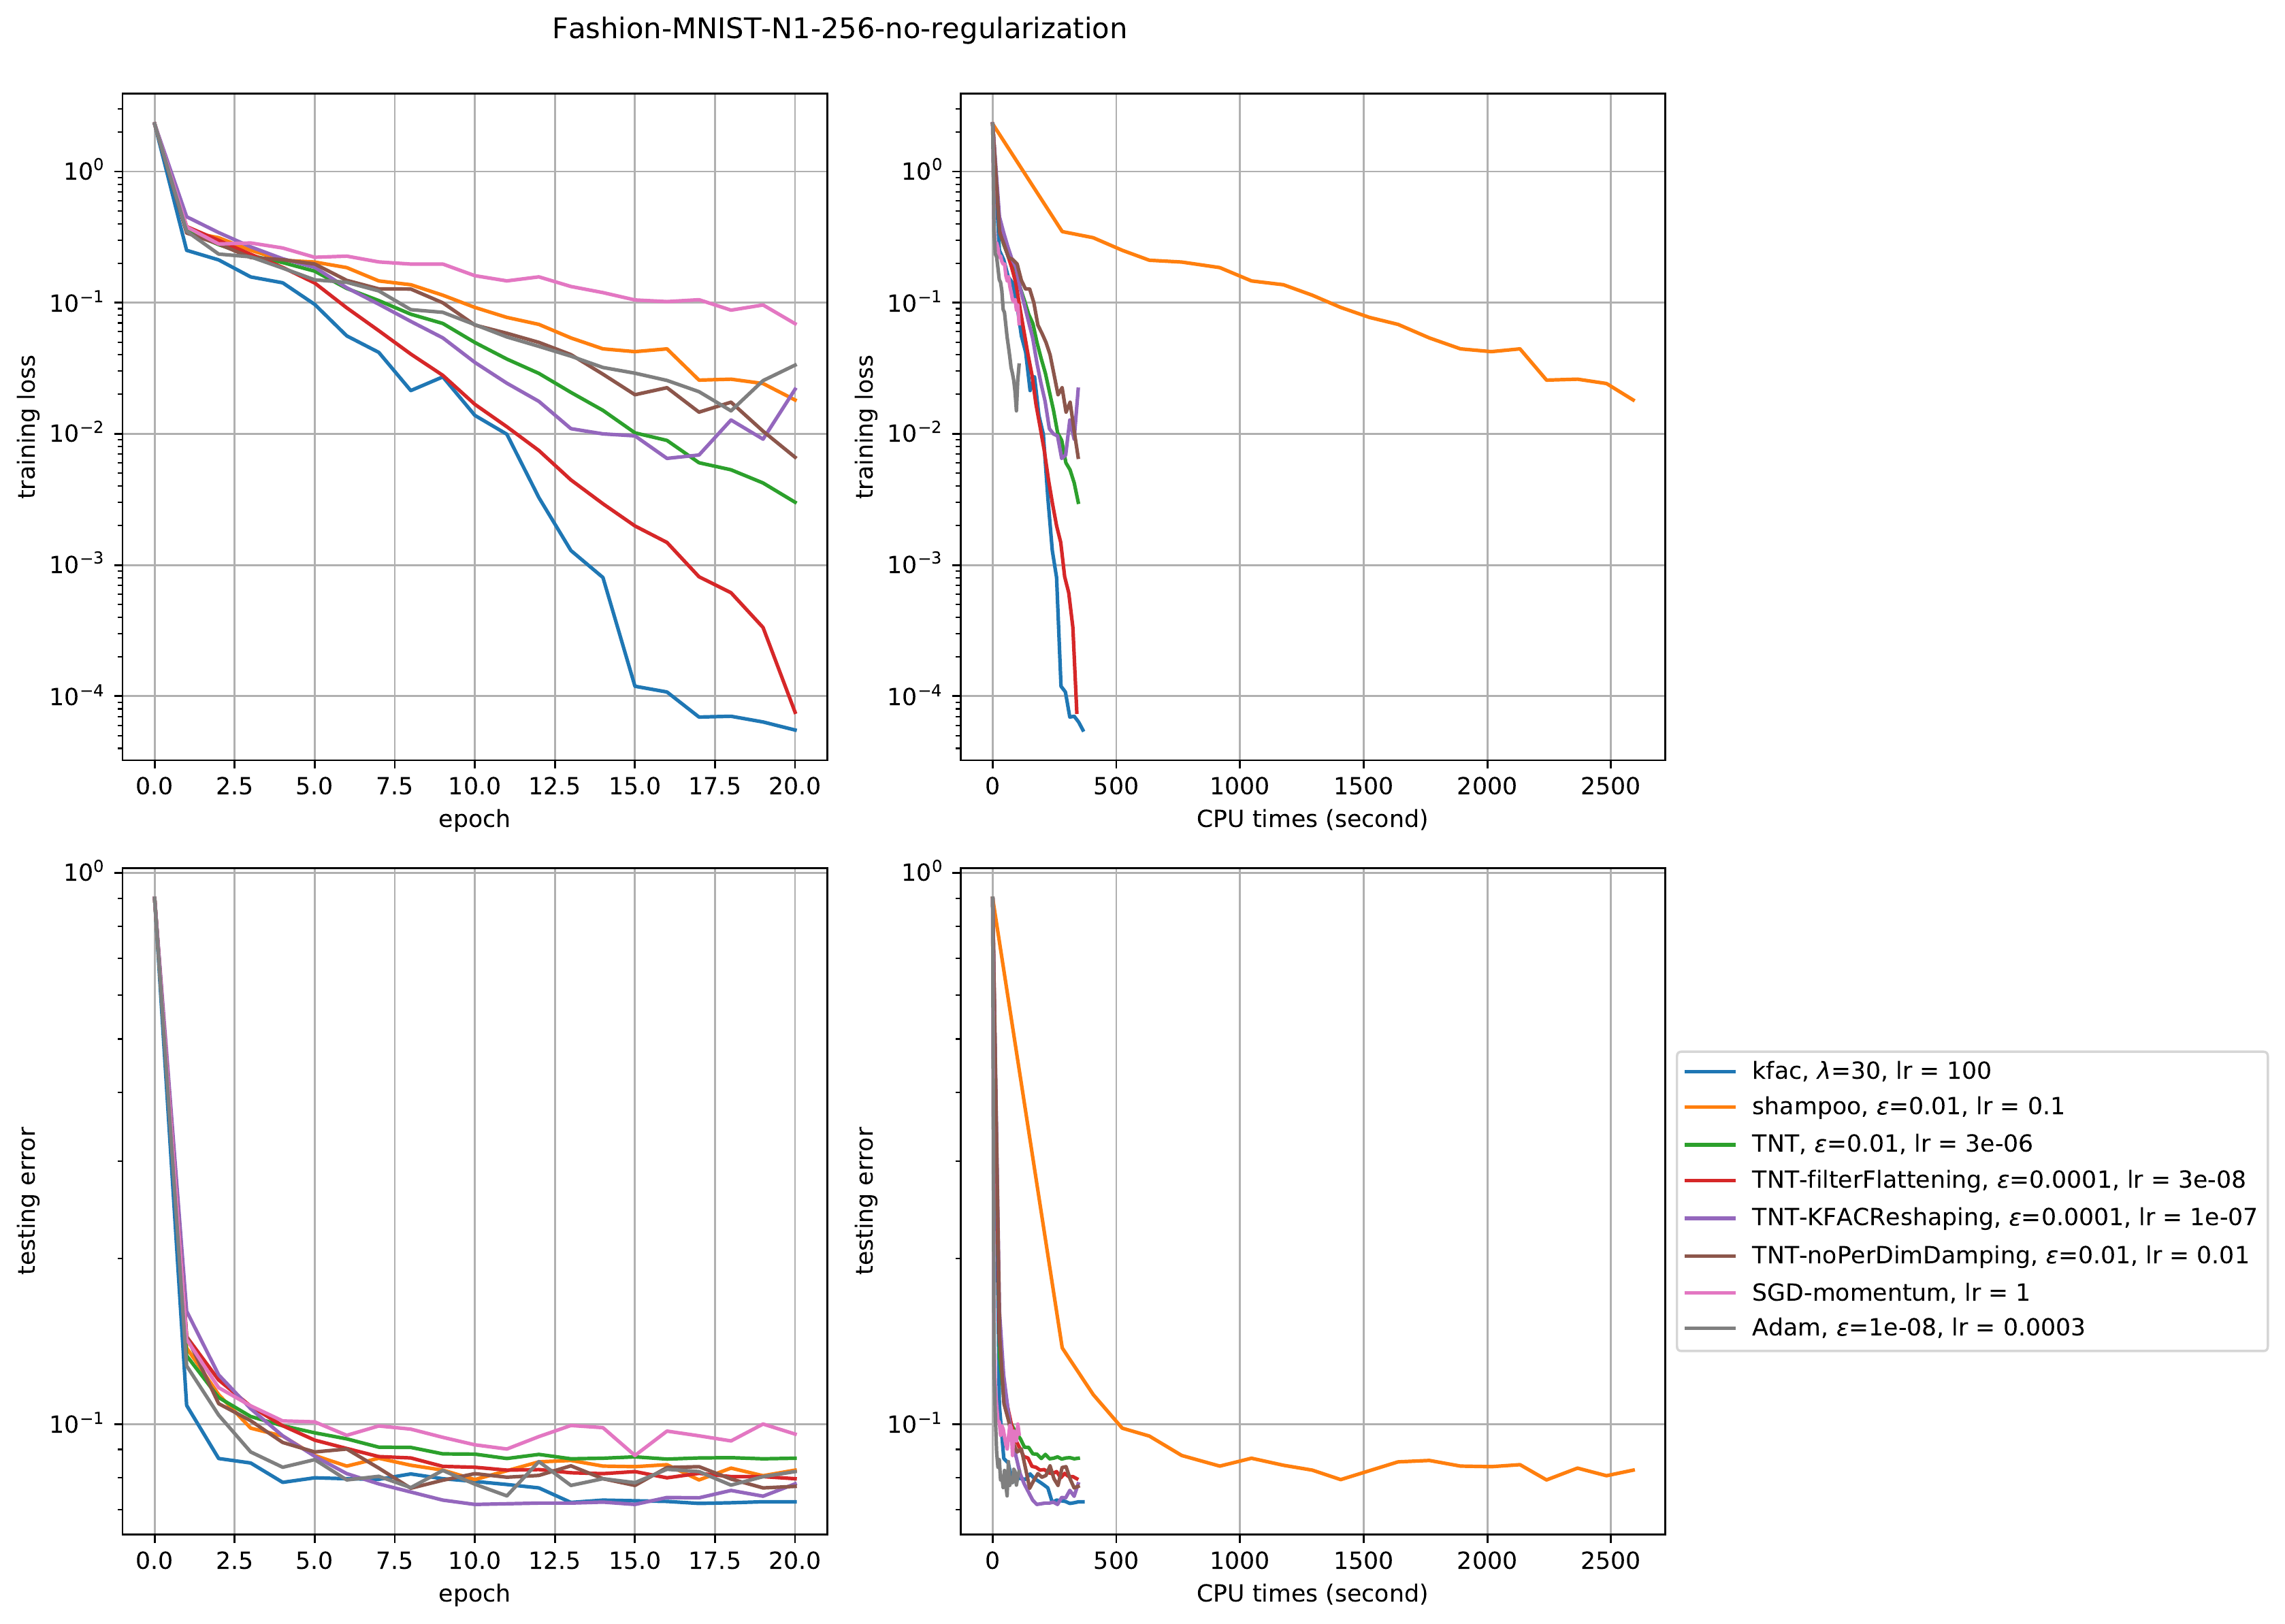}
    \caption{Fashion MNIST}
    \label{fig_2}
\end{figure}

\begin{figure}[H]
    \centering
    \includegraphics[width=\textwidth]{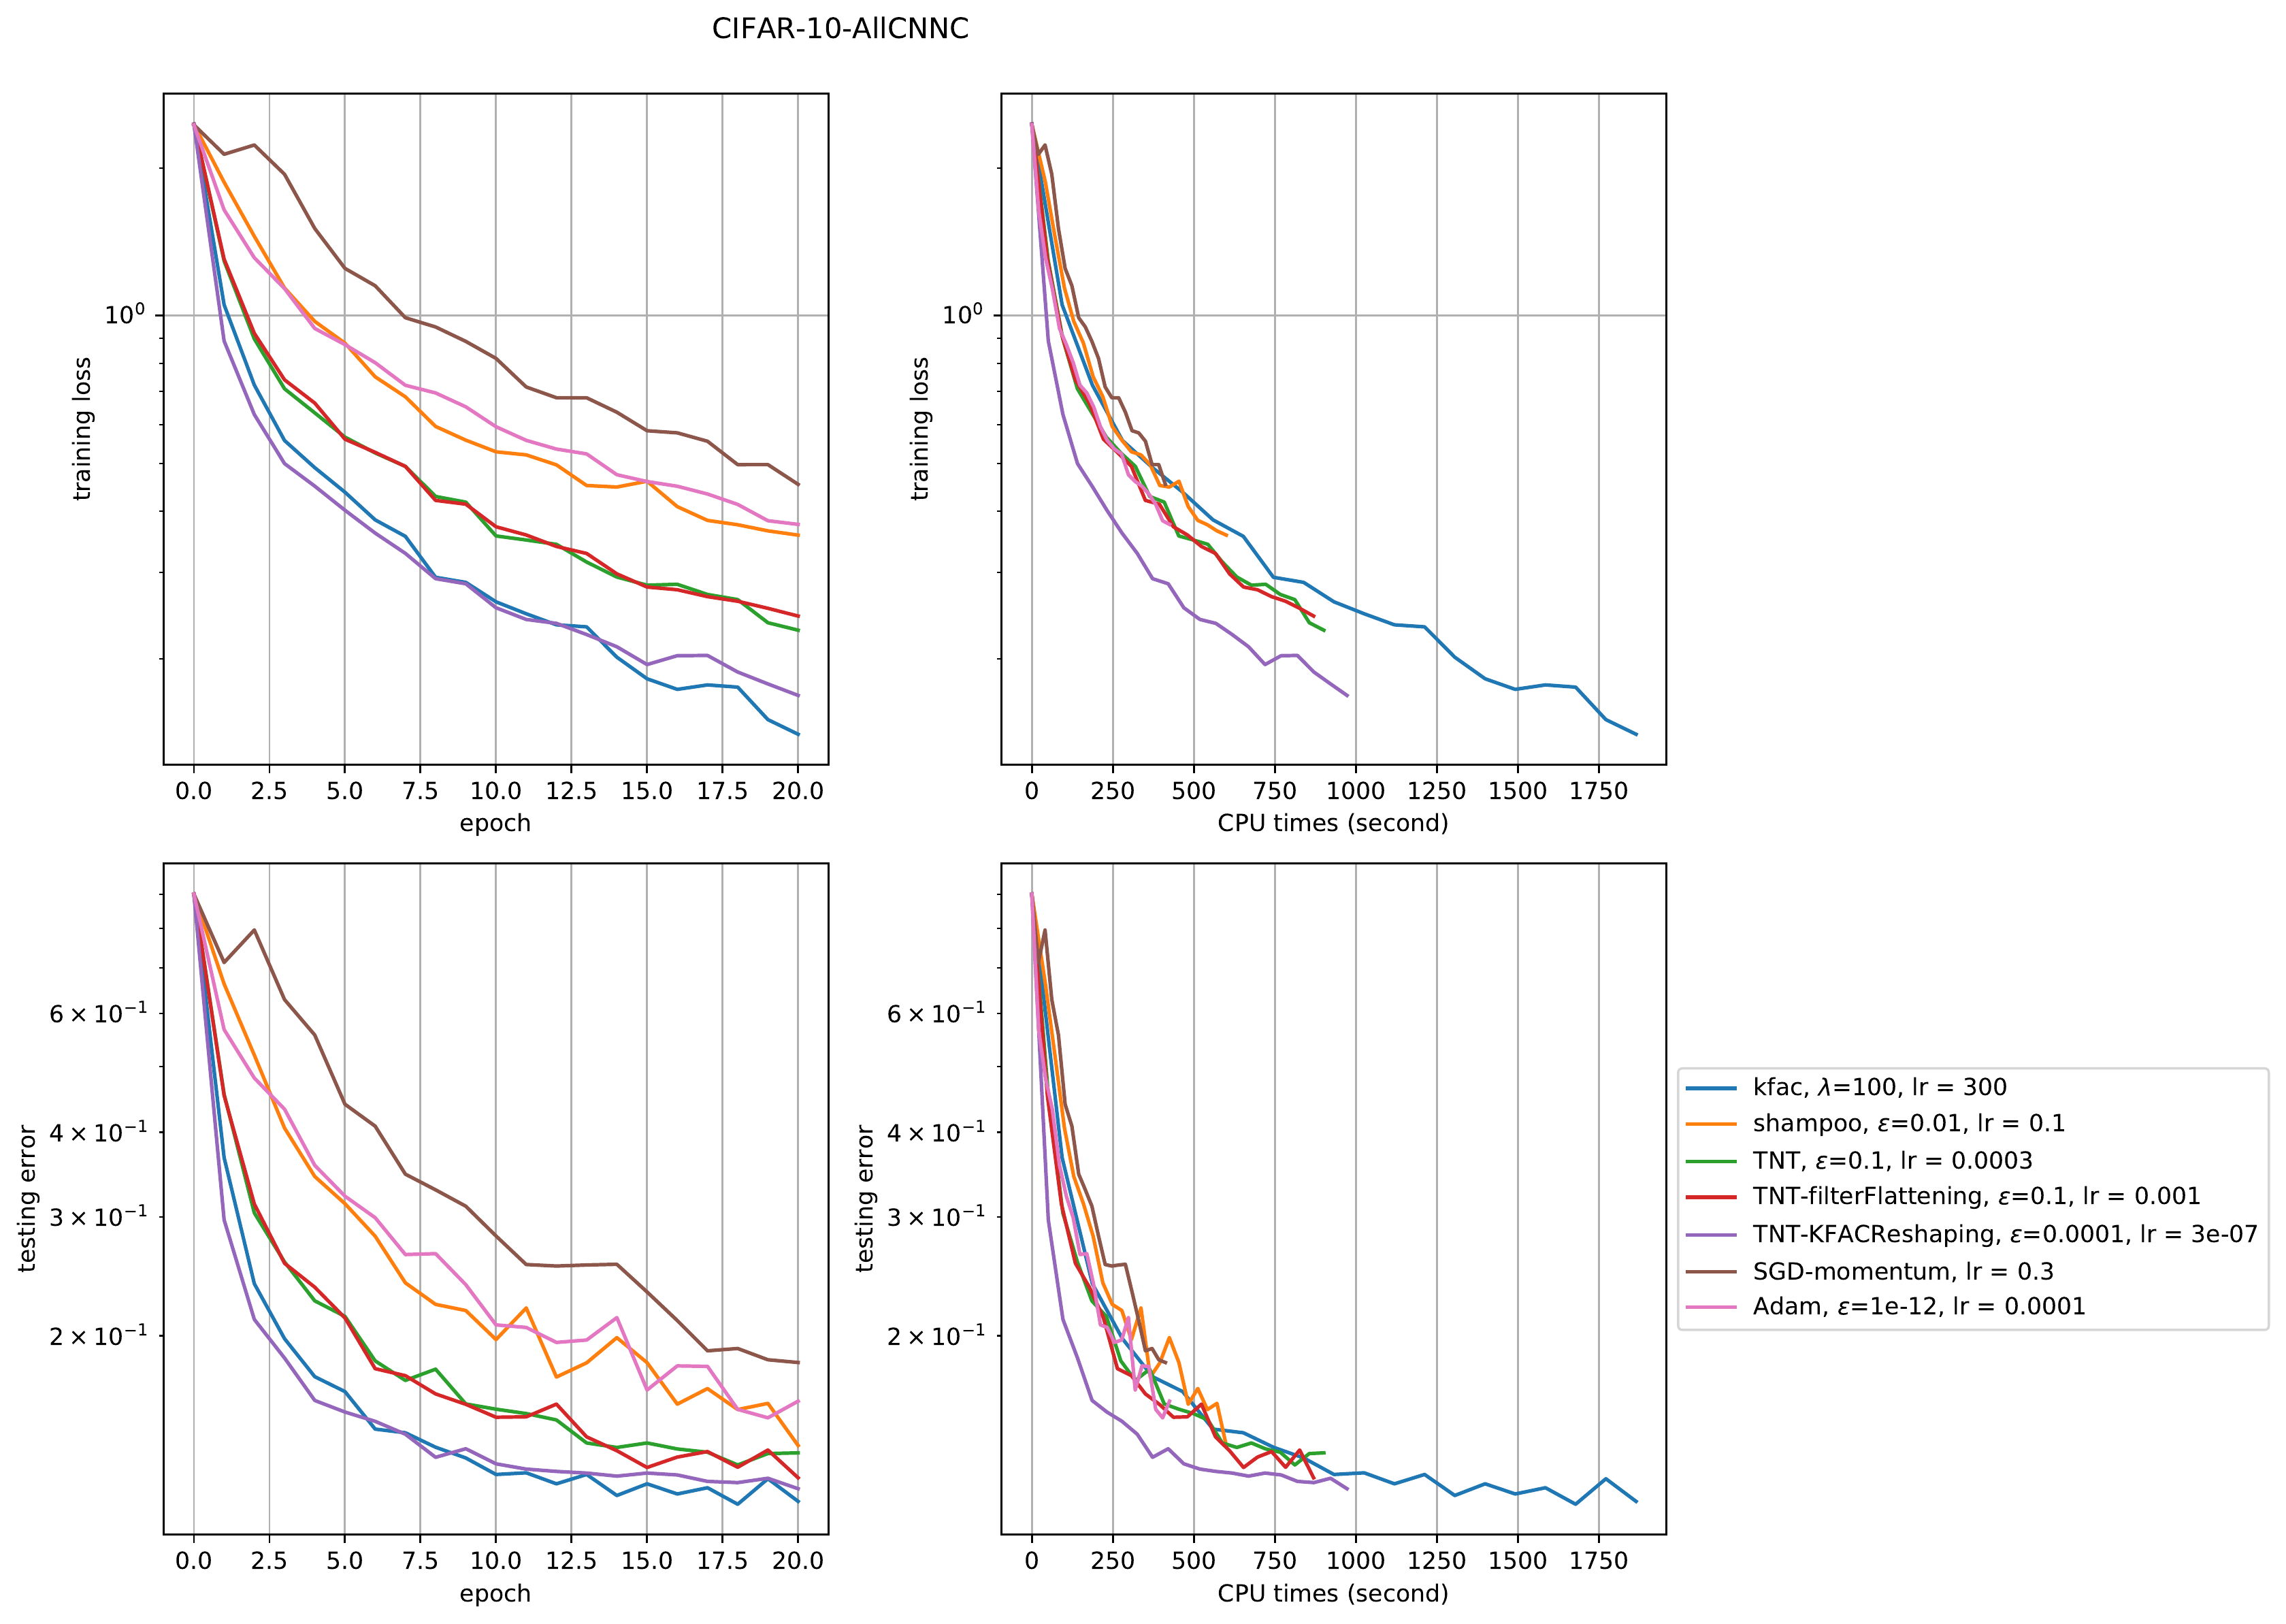}
    \caption{CIFAR-10, All-CNN-C}
    \label{fig_5}
\end{figure}

\begin{figure}[H]
    \centering
    \includegraphics[width=\textwidth]{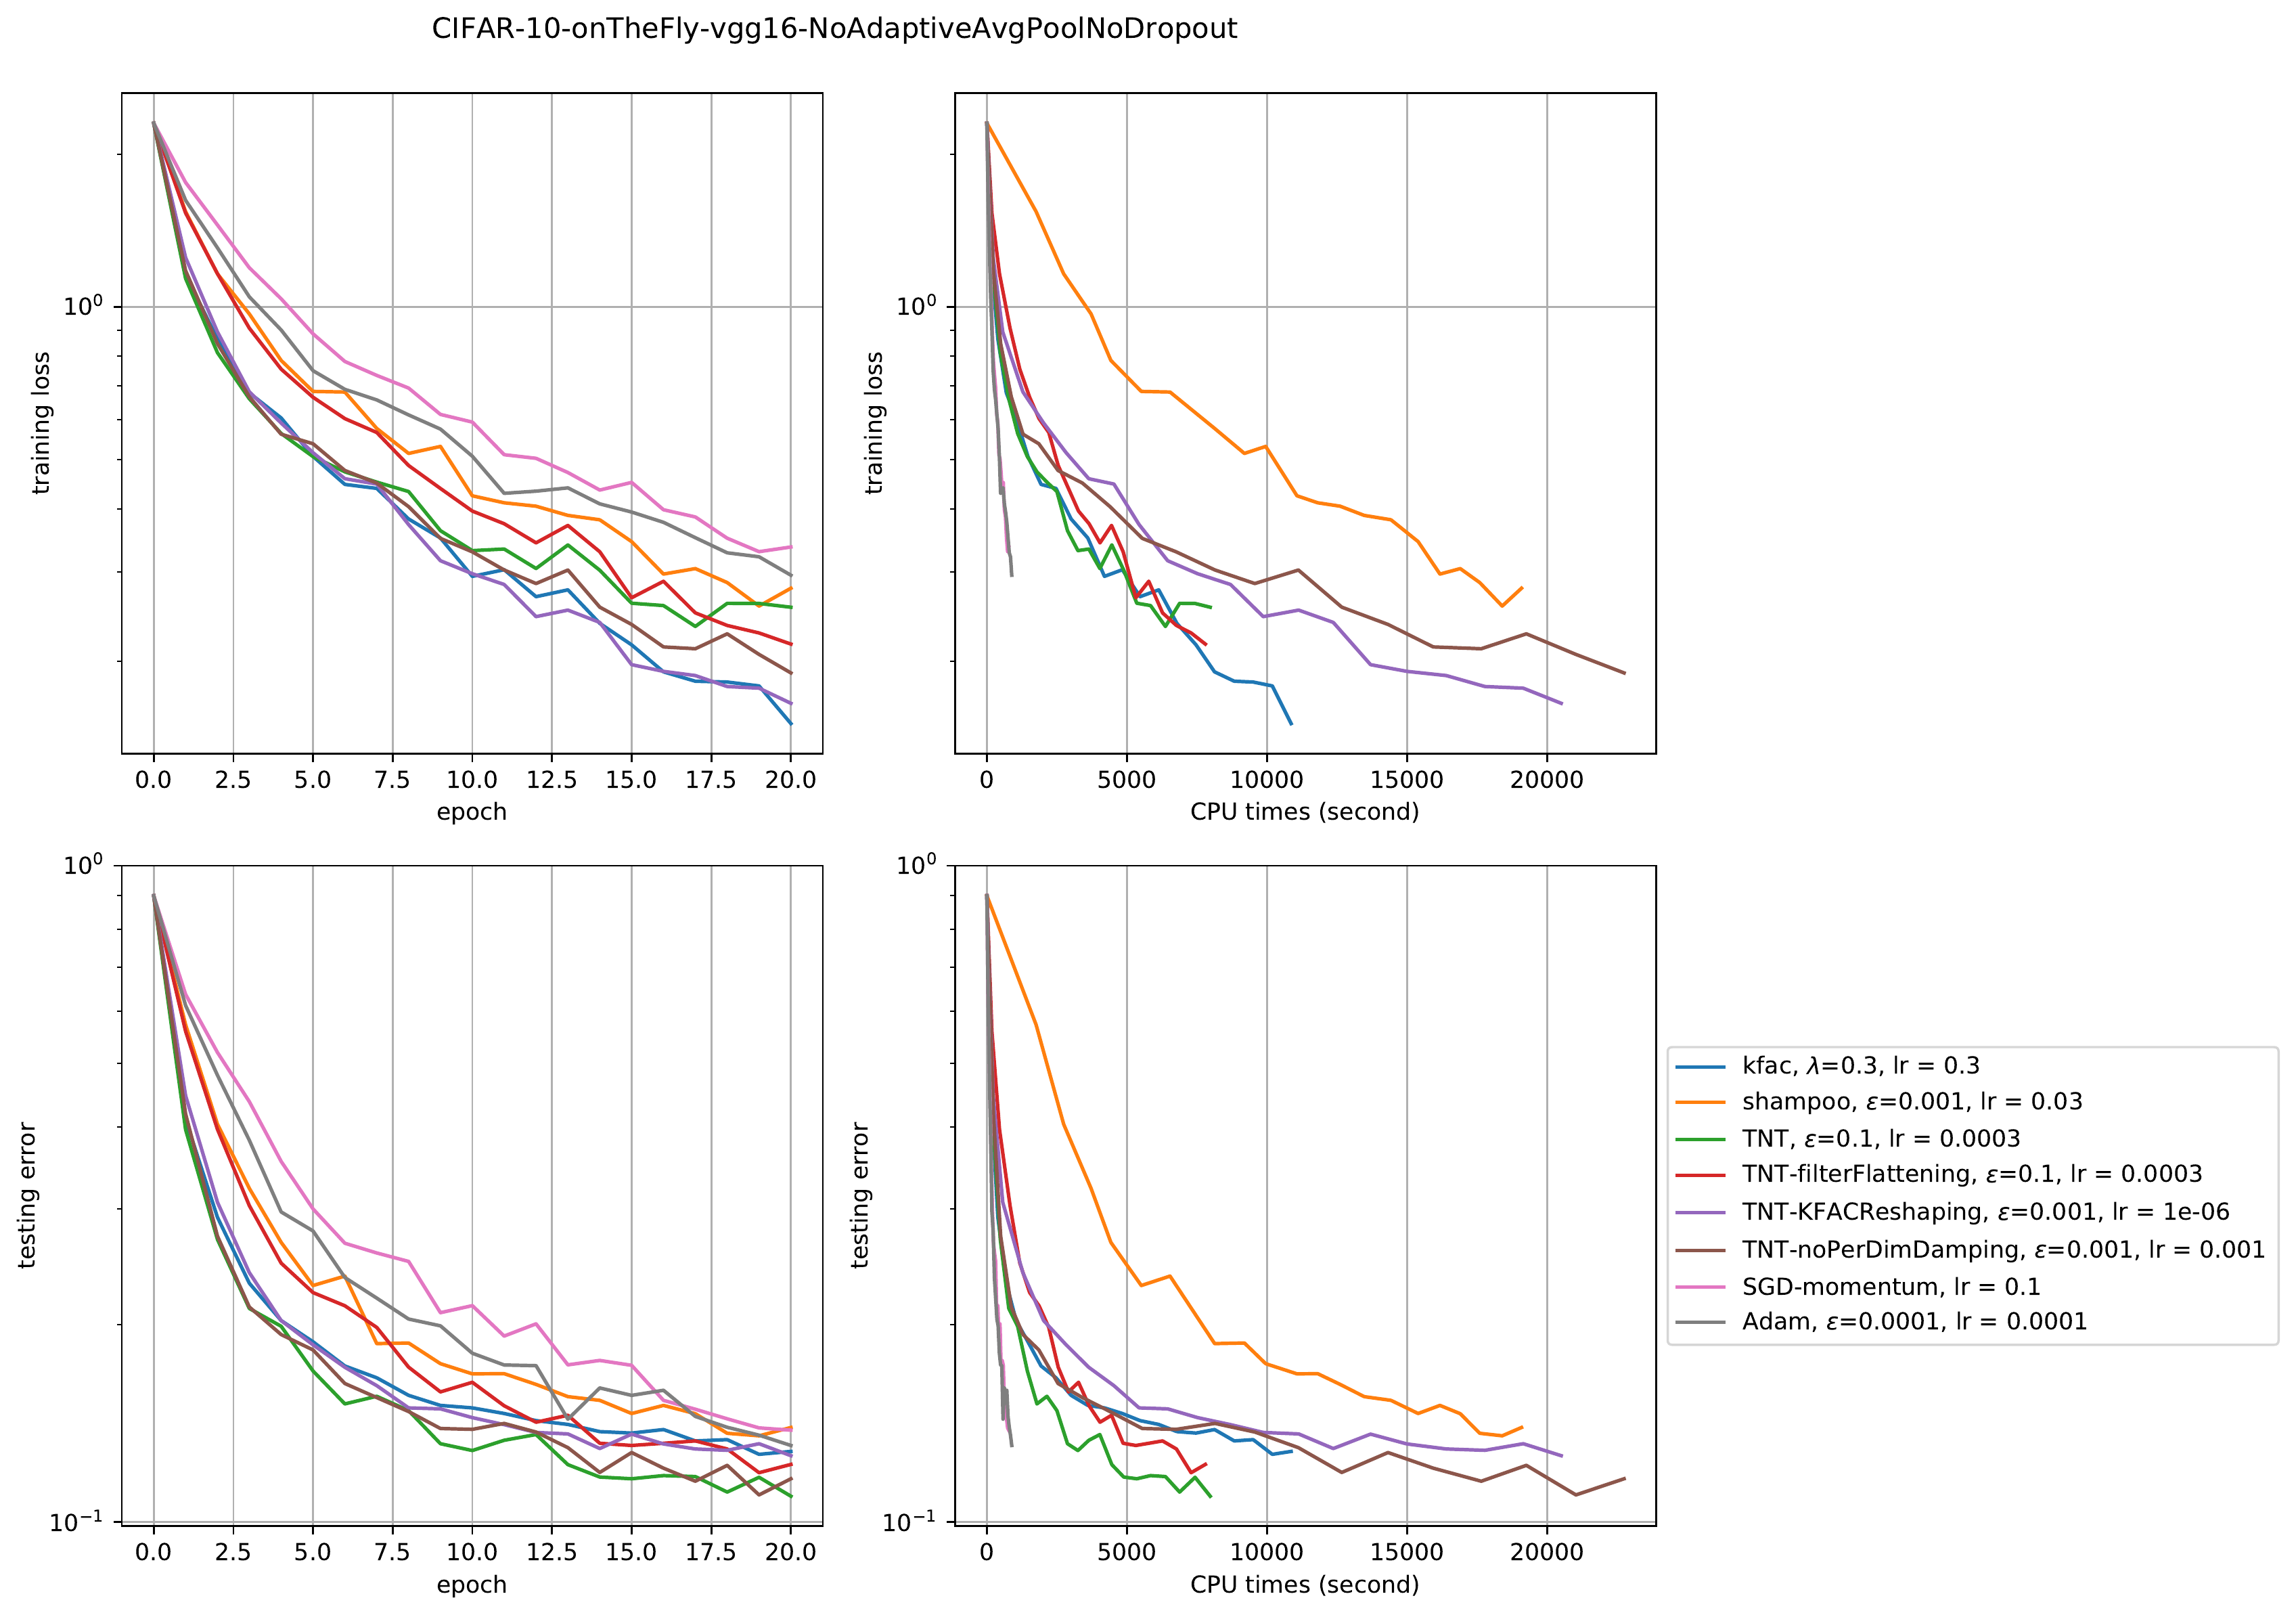}
    \caption{CIFAR-10, VGG16}
    \label{fig_4}
\end{figure}

\begin{figure}[H]
    \centering
    \includegraphics[width=\textwidth]{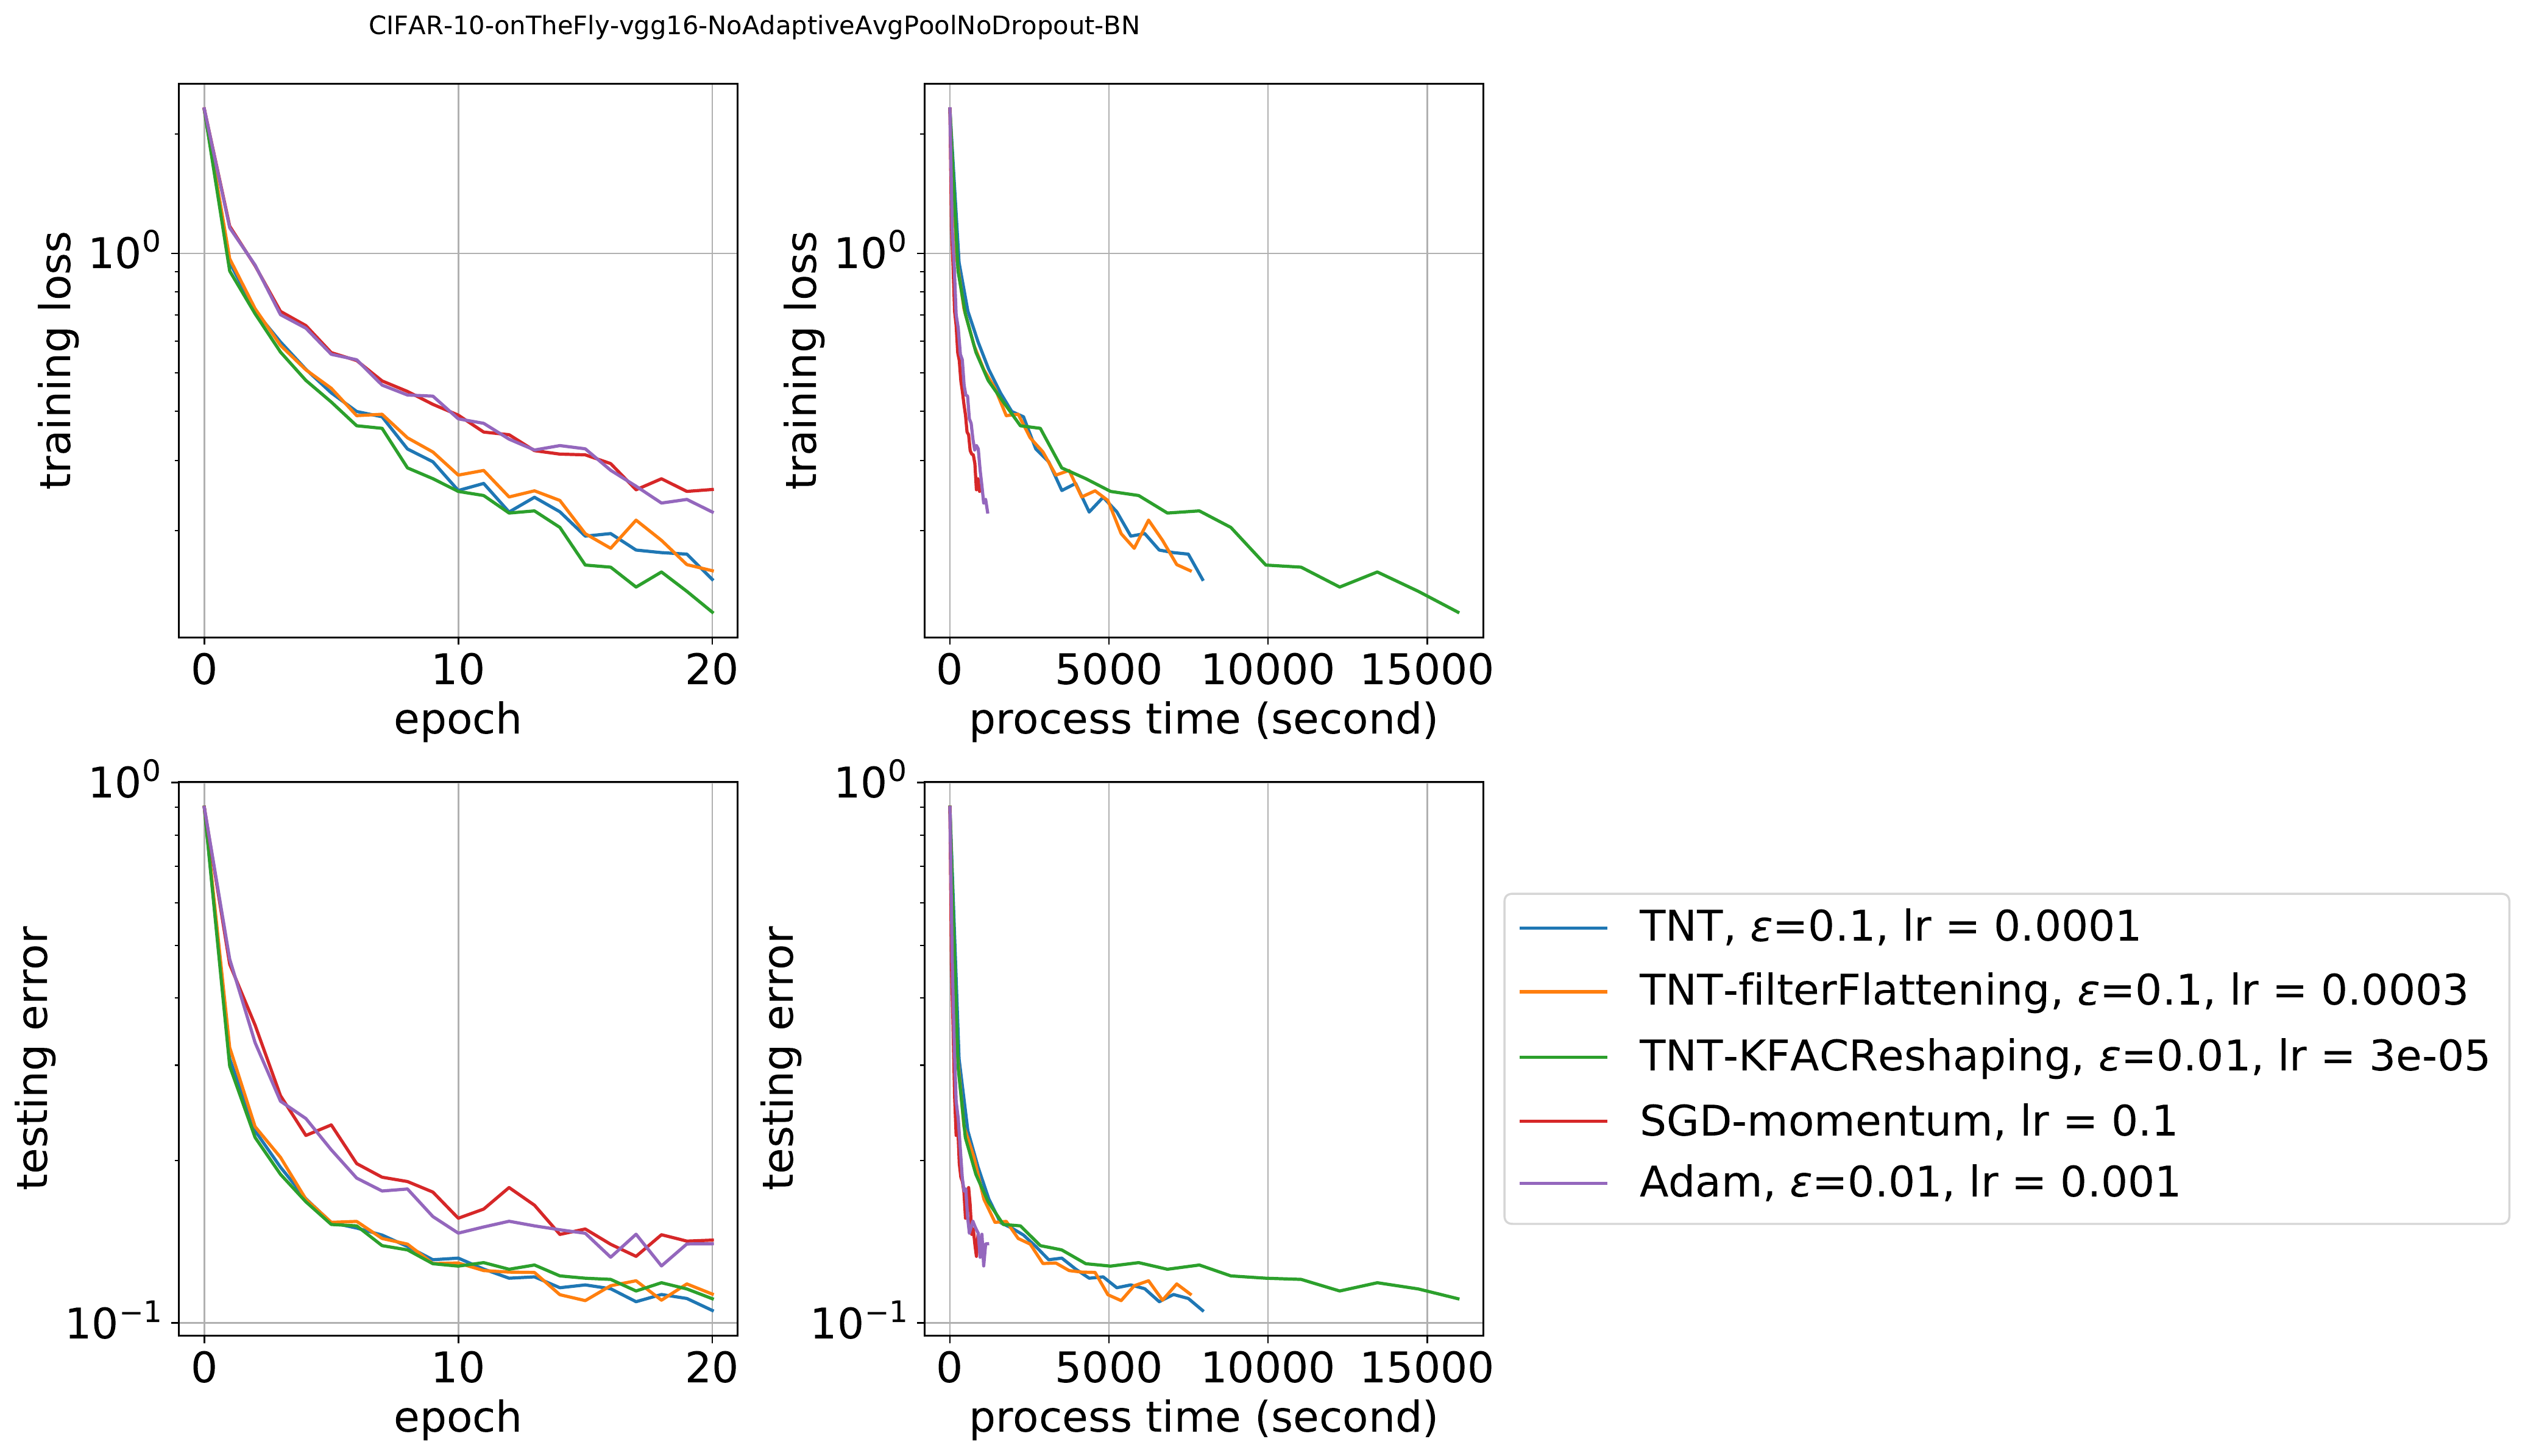}
    \caption{CIFAR-10, VGG16BN}
    \label{fig_6}
\end{figure}

\begin{figure}[H]
    \centering
    \includegraphics[width=\textwidth]{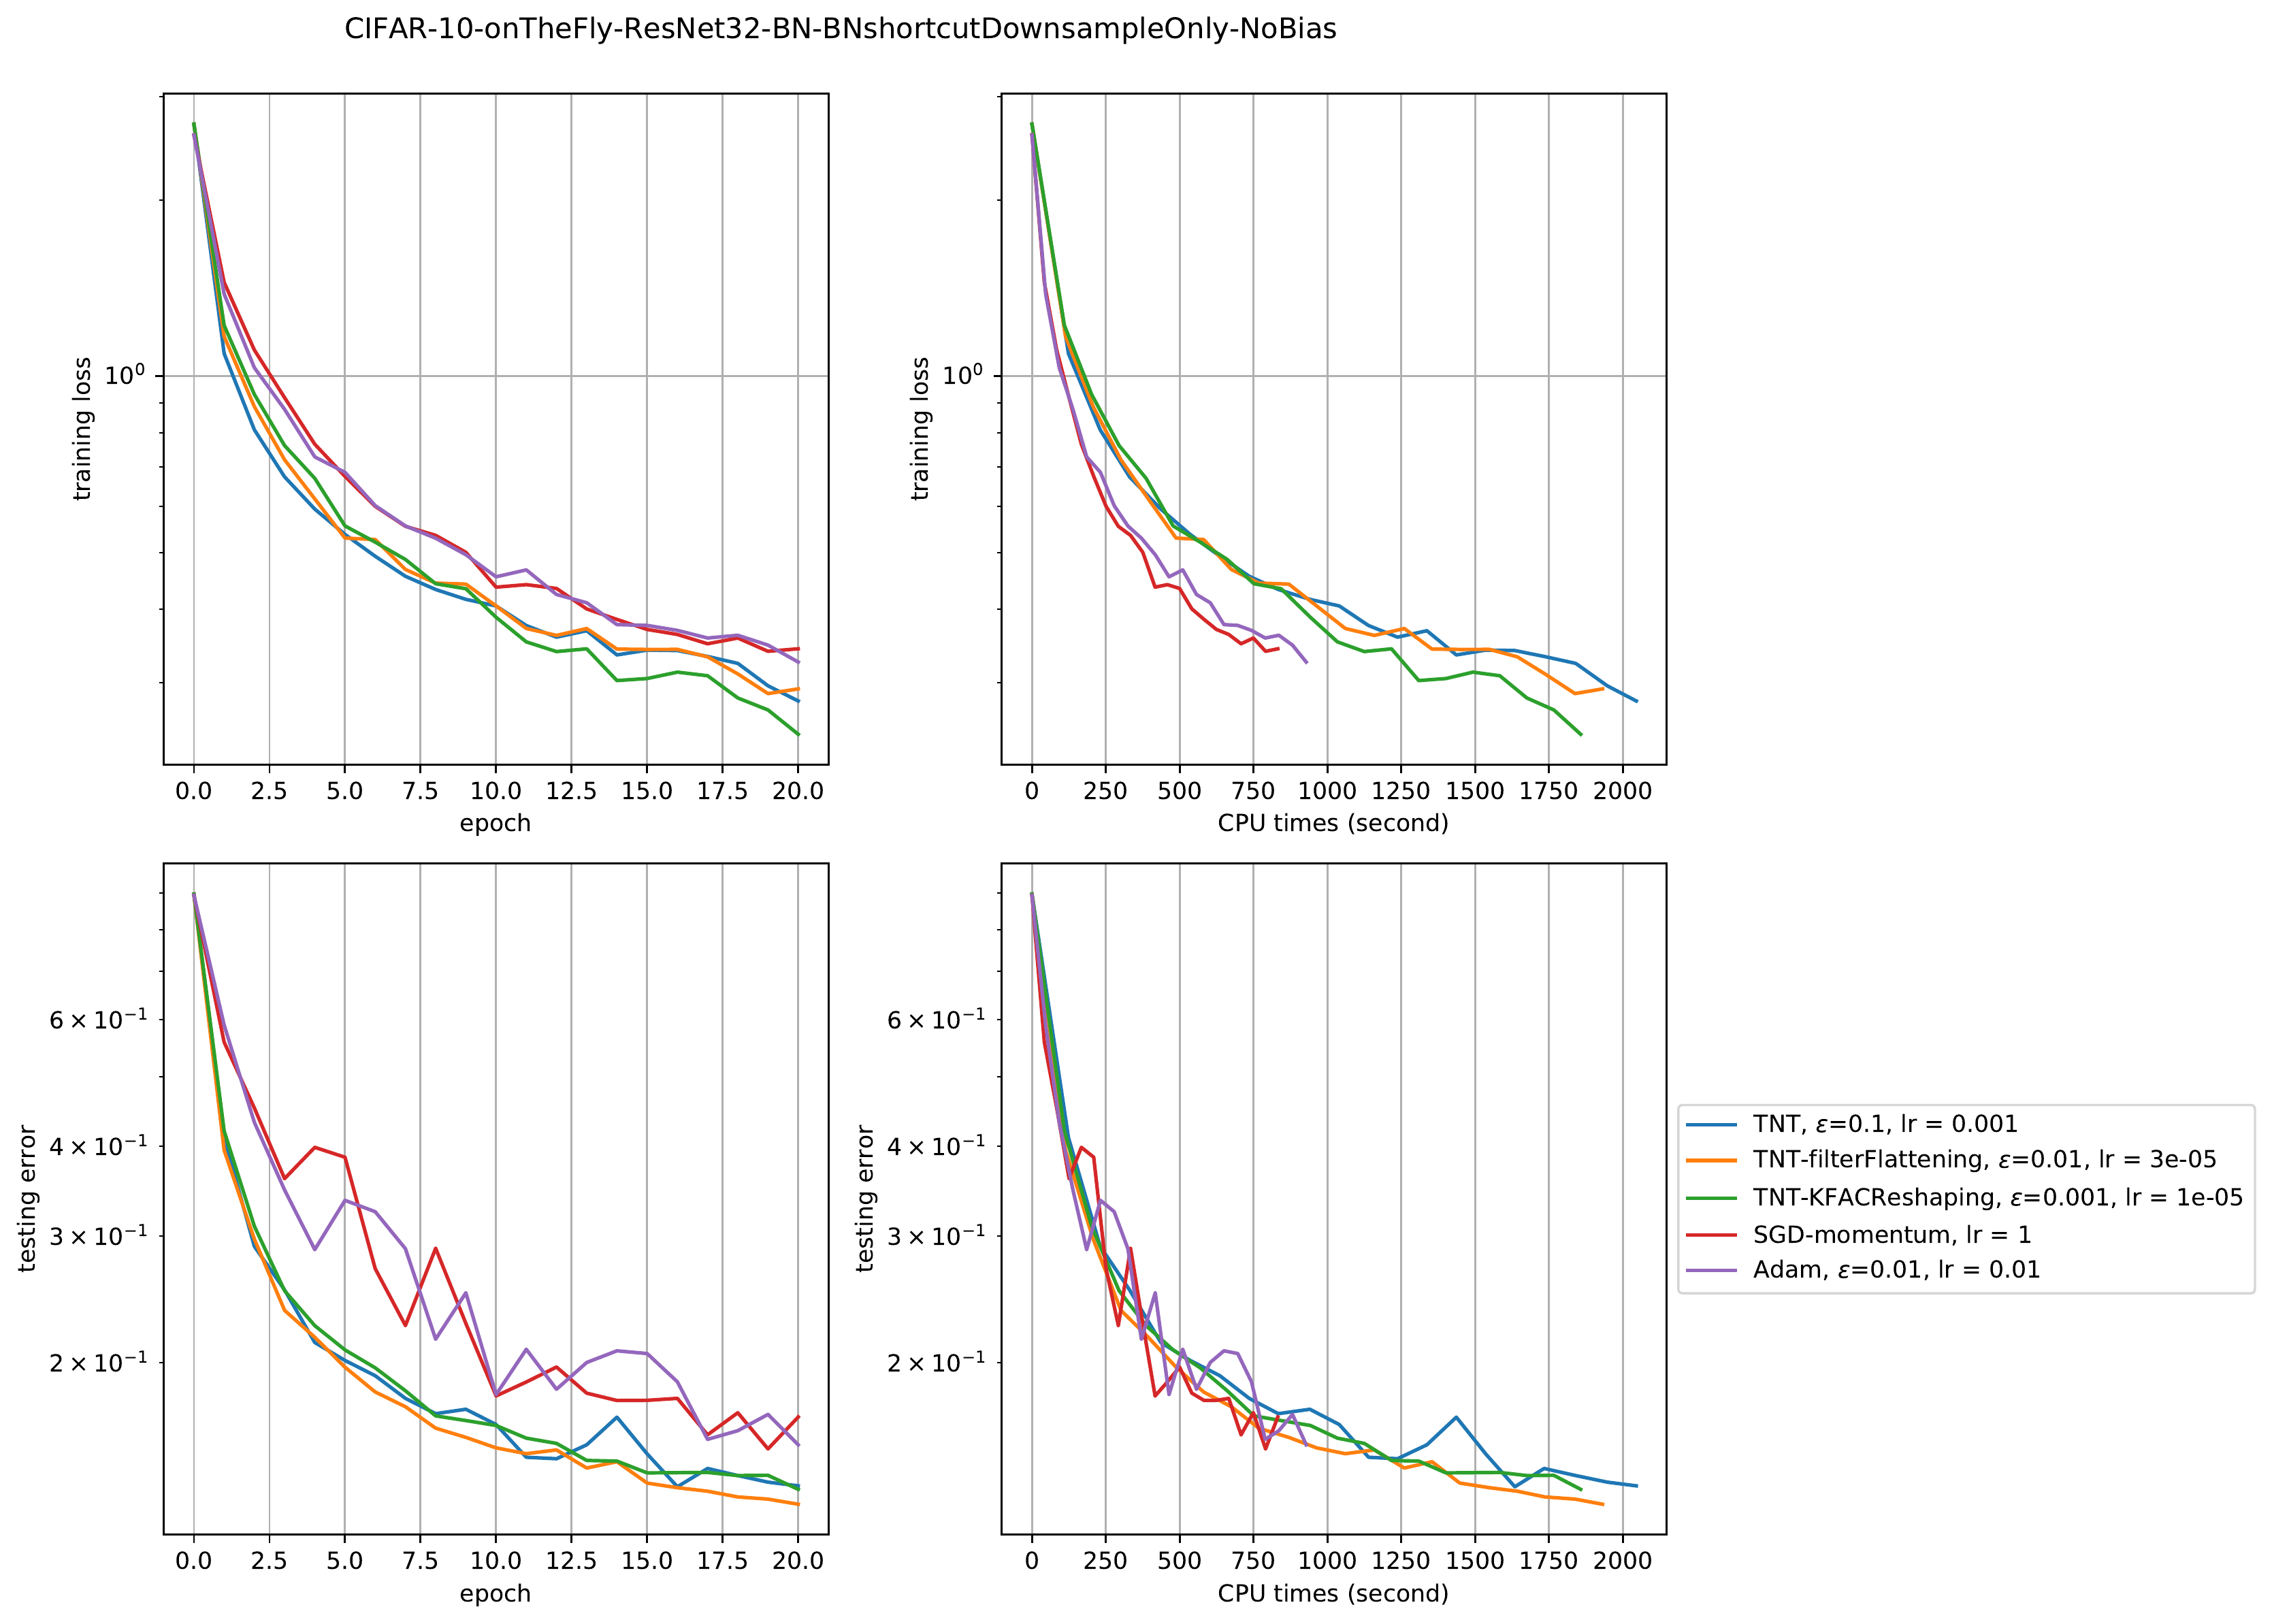}
    \caption{CIFAR-10, ResNet32}
    \label{fig_7}
\end{figure}
