# Supplementary material for: Tensor Normal Training for Deep Learning Models
Source: arXiv:2106.02925 source file (2021-12-21)
Supplement: Supplementary file 3 [file proof_not_used.tex]

\subsection{mimic \texorpdfstring{\cite{zhang2019fast}}{TEXT} (seems to be too complicated)}

\clarify{mimic \cite{zhang2019fast}}

We follow the notation in \cite{zhang2019fast}. 

Let $\theta \in \R^m$ denote all the parameters of the NN. Let $u$ denote the output of the NN. Let $i$ denote the index of a data-point. 

Because of the equivalence between Fisher matrix and Gauss-Newton matrix \clarify{(need reference)}, we have that the Fisher matrix $F = \E [J_i^\top H_i J_i]$, where $J_i$ is the Jacobian matrix of $u_i$ w.r.t $\theta$, $H_i$ is the Hessian w.r.t $u$. Since we use squared error loss \clarify{(how about other loss?)}, we have that $F = \E [J_i^\top J_i] = \frac{1}{n} J^\top J$, where $J = (J_1^\top, ..., J_n^\top)^\top$. 

\begin{lemma}
Expression of $F_{\text{TNT}}$ and $F_{\text{TNT}}^{-1}$:
\label{lemma_2}
\end{lemma}

% \ref{lemma_1}
% \ref{lemma_2} no

\begin{proof}

Since we assume that the NN has a single output \clarify{(how about multiple output?)}, we have that $J_i$ is of size $1 \times m$. We view $J_i$ as a random vector w.r.t $i$. Since $\E_i [J_i] = 0$ \clarify{(need to verify)}, we have that $F = \text{cov}_i (J_i)$. Since we assume that $J_i$ follows a matrix-normal distribution \clarify{(what about tensor normal?)} and that the NN has only one layer \clarify{(how about multiple layers?)}, we have that $F_{\text{TNT}} = U \otimes V$. 

Let $J_i = \text{vec}(G_i)$, by (\ref{eq_4}) and (\ref{eq_5}), we have that
\begin{align*}
    \mathbb{E}_i (G_i G_i^\top) = V \cdot \text{tr}(U),
    \\
    \mathbb{E}_i (G_i^\top G_i) = U \cdot \text{tr}(V).
\end{align*}
Thus,
\begin{align*}
    F_{\text{TNT}}
    = \frac{\mathbb{E}_i (G_i^\top G_i)}{\text{tr}(V)} \otimes \frac{\mathbb{E}_i (G_i G_i^\top)}{\text{tr}(U)}
    = \frac{1}{\text{tr}(V) \text{tr}(U)} \mathbb{E}_i (G_i^\top G_i) \otimes \mathbb{E}_i (G_i G_i^\top).
\end{align*}

If we assume that $J_i^\top = a_i \otimes g_i$ where $a_i$ and $g_i$ are $x_i$ and $\phi'(w x_i)$ in \cite{zhang2019fast}, respectively, \clarify{(what if we don't assume this)} we have that $G_i = g_i a_i^\top$. Thus
$G_i^\top G_i = (g_i^\top g_i) a_i a_i^\top := \tilde{a}_i \tilde{a}_i^\top$ where $\tilde{a}_i = ||g_i|| a_i$.
Similarly, $G_i G_i^\top = (a_i^\top a_i) g_i g_i^\top := \tilde{g}_i \tilde{g}_i^\top$ where $\tilde{g}_i = ||a_i|| g_i$. 

Hence, \clarify{kfac handles the expectation wrongly?}
\begin{align*}
    \mathbb{E}_i (G_i^\top G_i)
    = \mathbb{E}_i ( \tilde{a}_i \tilde{a}_i^\top )
    = \frac{1}{n} \sum_{i=1}^n \tilde{a}_i \tilde{a}_i^\top
    := \frac{1}{n} \tilde{X}^\top \tilde{X},
\end{align*}
where $\tilde{X} = (\tilde{a}_1, ..., \tilde{a}_n)^\top \in \R^{n \times d}$. Similarly, $\mathbb{E}_i (G_i G_i^\top) = \frac{1}{n} \tilde{S}^\top \tilde{S}$ where $\tilde{S} = (\tilde{g}_1, ..., \tilde{g}_n)^\top \in \R^{n \times m}$. Also, 
\begin{align*}
    \text{tr}(V) \text{tr}(U)
    & = \text{tr} \left( \mathbb{E}_i (G_i G_i^\top) \right)
    = \mathbb{E}_i \left( \text{tr} \left( G_i G_i^\top \right) \right)
    = \mathbb{E}_i \left( \text{tr} \left( (a_i^\top a_i) g_i g_i^\top \right) \right)
    = \mathbb{E}_i \left( (a_i^\top a_i) (g_i^\top g_i) \right)
    \\
    & = \frac{1}{n} \sum_{i=1}^n ||a_i||^2 ||g_i||^2
\end{align*}
Thus,
\begin{align*}
    F_{\text{TNT}}
    = \frac{n}{\sum_{i=1}^n ||a_i||^2 ||g_i||^2} \left( \frac{1}{n} \tilde{X}^\top \tilde{X} \right) \otimes \left( \frac{1}{n} \tilde{S}^\top \tilde{S} \right)
    = \frac{1}{n \sum_{i=1}^n ||a_i||^2 ||g_i||^2} \left( \tilde{X}^\top \tilde{X} \right) \otimes \left( \tilde{S}^\top \tilde{S} \right).
\end{align*}

Hence,
\begin{align*}
    F_{\text{TNT}}^{-1}
    = n \sum_{i=1}^n ||a_i||^2 ||g_i||^2 \left( \tilde{X}^\top \tilde{X} \right)^{-1} \otimes \left( \tilde{S}^\top \tilde{S} \right)^{-1}.
\end{align*}
Note that we assume $d < n < m$ \clarify{(what if we don't)}, $\tilde{S}^\top \tilde{S}$ is not full-rank, and hence $( \tilde{S}^\top \tilde{S} )^{-1}$ is generalized inverse.

\end{proof}

\begin{lemma}
\label{lemma_1}
\end{lemma}

% \ref{lemma_1}

\begin{proof}

% \deletethis{
% \begin{align*}
%     &\mathbf{u}(k+1)-\mathbf{u}(k)
%     \\
%     =& \mathbf{u}\left(\mathbf{w}(k)-\eta \mathbf{F}_{\text{TNT}}^{-1}(k) \mathbf{J}(k)^{\top}(\mathbf{u}(k)-\mathbf{y})\right)-\mathbf{u}(\mathbf{w}(k))
%     \\
%     & \text{(because $\frac{\partial L}{\partial \theta} = J^\top (\vu - \vy)$ \clarify{should have $\frac{1}{n}$; can we relax this?})}
%     \\
%     =&-\int_{s=0}^{1}\left\langle\frac{\partial \mathbf{u}(\mathbf{w}(s))}{\partial \mathbf{w}^{\top}}, \eta \mathbf{F}_{\text{TNT}}^{-1}(k) \mathbf{J}(k)^{\top}(\mathbf{u}(k)-\mathbf{y})\right\rangle d s 
%     \\
%     =&-\int_{s=0}^{1}\left\langle\frac{\partial \mathbf{u}(\mathbf{w}(k))}{\partial \mathbf{w}^{\top}}, \eta \mathbf{F}_{\text{TNT}}^{-1}(k) \mathbf{J}(k)^{\top}(\mathbf{u}(k)-\mathbf{y})\right\rangle d s \\ &+\int_{s=0}^{1}\left\langle\frac{\partial \mathbf{u}(\mathbf{w}(k))}{\partial \mathbf{w}^{\top}}-\frac{\partial \mathbf{u}(\mathbf{w}(s))}{\partial \mathbf{w}^{\top}}, \eta \mathbf{F}_{\text{TNT}}^{-1}(k) \mathbf{J}(k)^{\top}(\mathbf{u}(k)-\mathbf{y})\right) d s
%     \\
%     & := \text{\textcircled{1}} + \text{\textcircled{2}}
% \end{align*}
% }

\addthis{
\begin{align*}
    &\mathbf{u}(k+1)-\mathbf{u}(k)
    \\
    =& \mathbf{u} \left( \mathbf{w}(k) - \eta \mathbf{F}_{\text{TNT}}^{-1}(k) \frac{1}{n} \mathbf{J}(k)^{\top}(\mathbf{u}(k)-\mathbf{y}) \right) - \mathbf{u}(\mathbf{w}(k))
    \\
    & \text{(because $\frac{\partial L}{\partial \theta} = \frac{1}{n} J^\top (\vu - \vy)$ \clarify{kfac handle the expectation wrongly?; can we relax this?})}
    \\
    = & -\int_{s=0}^{1}\left\langle\frac{\partial \mathbf{u}(\mathbf{w}(s))}{\partial \mathbf{w}^{\top}}, \eta \mathbf{F}_{\text{TNT}}^{-1}(k) \frac{1}{n} \mathbf{J}(k)^{\top}(\mathbf{u}(k)-\mathbf{y})\right\rangle d s 
    \\
    = & -\int_{s=0}^{1}\left\langle\frac{\partial \mathbf{u}(\mathbf{w}(k))}{\partial \mathbf{w}^{\top}}, \eta \mathbf{F}_{\text{TNT}}^{-1}(k) \frac{1}{n} \mathbf{J}(k)^{\top}(\mathbf{u}(k)-\mathbf{y})\right\rangle d s \\ &+\int_{s=0}^{1}\left\langle\frac{\partial \mathbf{u}(\mathbf{w}(k))}{\partial \mathbf{w}^{\top}}-\frac{\partial \mathbf{u}(\mathbf{w}(s))}{\partial \mathbf{w}^{\top}}, \eta \mathbf{F}_{\text{TNT}}^{-1}(k) \frac{1}{n} \mathbf{J}(k)^{\top}(\mathbf{u}(k)-\mathbf{y})\right) d s
    \\
    & := \text{\textcircled{1}} + \text{\textcircled{2}}
\end{align*}
}

We first claim that \textcircled{2} is negligible \clarify{(need to verify)}. As for \textcircled{1},
\begin{align*}
    \text{\textcircled{1}} = \eta \mathbf{J}(k) \mathbf{F}_{\text{TNT}}^{-1}(k) \frac{1}{n} \mathbf{J}(k)^\top (\vy - \vu(k)).
\end{align*}
Hence, 
\begin{align*}
    \mathbf{u}(k+1)-\mathbf{u}(k)
    & \approx \eta \mathbf{J}(k) \mathbf{F}_{\text{TNT}}^{-1}(k) \frac{1}{n} \mathbf{J}(k)^\top (\vy - \vu(k))
    \\
    & = \eta (X * S) \left( n \sum_{i=1}^n ||a_i||^2 ||g_i||^2 \left( \tilde{X}^\top \tilde{X} \right)^{-1} \otimes \left( \tilde{S}^\top \tilde{S} \right)^{-1} \right) \frac{1}{n} (X^\top * S^\top) (\vy - \vu(k))
    \\
    & \text{(because $J(k) = X * S$ \clarify{(what if we don't assume this)} and Lemma \ref{lemma_2})}
    \\
    & = \eta \sum_{i=1}^n ||a_i||^2 ||g_i||^2 (\widecheck{X} * \tilde{S}) \left( \left( \tilde{X}^\top \tilde{X} \right)^{-1} \otimes \left( \tilde{S}^\top \tilde{S} \right)^{-1} \right) (\widecheck{X}^\top * \tilde{S}^\top) (\vy - \vu(k))
    \\
    & \text{($\widecheck{X} := (\widecheck{a}_1, ..., \widecheck{a}_n)^\top$ and $\widecheck{a_i} := \frac{1}{||a_i||} a_i$)}
    \\
    & = \eta \sum_{i=1}^n ||a_i||^2 ||g_i||^2 \left( \left( \widecheck{X} \left( \tilde{X}^\top \tilde{X} \right)^{-1} \widecheck{X}^\top \right) \odot \left( \tilde{S} \left( \tilde{S}^\top \tilde{S} \right)^{-1} \tilde{S}^\top \right) \right) (\vy - \vu(k))
    \\
    & = \eta \sum_{i=1}^n ||a_i||^2 ||g_i||^2 \left( \left( \widecheck{X} \left( \tilde{X}^\top \tilde{X} \right)^{-1} \widecheck{X}^\top \right) \odot I \right) (\vy - \vu(k))
\end{align*}

\end{proof}

\begin{lemma}
\label{lemma_3}
\end{lemma}

% \ref{lemma_1}
% \ref{lemma_2}
% \ref{lemma_3} no
% \ref{lemma_4} no

\begin{proof}

Let $i^* = \text{argmin}_i \left( \widecheck{X} \left( \tilde{X}^\top \tilde{X} \right)^{-1} \widecheck{X}^\top \right)_{ii}$. Thus,
\begin{align*}
    & \ve_{i^*}^\top \left( \widecheck{X} \left( \tilde{X}^\top \tilde{X} \right)^{-1} \widecheck{X}^\top \right) \ve_{i^*}
    = \min_i \left( \widecheck{X} \left( \tilde{X}^\top \tilde{X} \right)^{-1} \widecheck{X}^\top \right)_{ii}
    \\
    \Leftrightarrow & 
    \widecheck{a}_{i^*}^\top \left( \tilde{X}^\top \tilde{X} \right)^{-1} \widecheck{a}_{i^*}
    = \min_i \left( \widecheck{X} \left( \tilde{X}^\top \tilde{X} \right)^{-1} \widecheck{X}^\top \right)_{ii}
    \\
    \Rightarrow &
    \lambda_{\min} \left\{ \left( \tilde{X}^\top \tilde{X} \right)^{-1} \right\} = \lambda_{\min} \left\{ \left( \tilde{X}^\top \tilde{X} \right)^{-1} \right\} ||\widecheck{a}_{i^*}||^2
    \le \widecheck{a}_{i^*}^\top \left( \tilde{X}^\top \tilde{X} \right)^{-1} \widecheck{a}_{i^*}
    \\ & 
    = \min_i \left( \widecheck{X} \left( \tilde{X}^\top \tilde{X} \right)^{-1} \widecheck{X}^\top \right)_{ii}.
\end{align*}

Thus,
\begin{align*}
    & \lambda_{\min} \left\{ \left( \widecheck{X} \left( \tilde{X}^\top \tilde{X} \right)^{-1} \widecheck{X}^\top \right) \odot I \right\}
    \ge \min_i \left( \widecheck{X} \left( \tilde{X}^\top \tilde{X} \right)^{-1} \widecheck{X}^\top \right)_{ii} \lambda_{\min}(I)
    \\
    \ge & \lambda_{\min} \left\{ \left( \tilde{X}^\top \tilde{X} \right)^{-1} \right\} = \frac{1}{\lambda_{\max} \left\{ \tilde{X}^\top \tilde{X} \right\} }.
\end{align*}

\end{proof}

\begin{lemma}
\label{lemma_4}
\end{lemma}

% \ref{lemma_1}
% \ref{lemma_2}
% \ref{lemma_3}
% \ref{lemma_4} no

\begin{proof}

\begin{align*}
    & \sum_{i=1}^n ||a_i||^2 ||g_i||^2 \cdot \frac{1}{\lambda_{\max} \left\{ \tilde{X}^\top \tilde{X} \right\} }
    \ge \frac{1}{\lambda_{\max} \left\{ {X}^\top {X} \right\} }
    \\
    \Leftrightarrow & \sum_{i=1}^n ||a_i||^2 ||g_i||^2 \cdot \lambda_{\max} \left\{ {X}^\top {X} \right\}
    \ge \lambda_{\max} \left\{ \tilde{X}^\top \tilde{X} \right\}
\end{align*}

For any vector $\vv$, 
\begin{align*}
    & \vv^\top \left( \sum_{i=1}^n ||a_i||^2 ||g_i||^2 \cdot {X}^\top {X} \right) \vv \ge \vv^\top \left( \tilde{X}^\top \tilde{X} \right) \vv
    \\
    \Leftrightarrow & \sum_{i=1}^n ||a_i||^2 ||g_i||^2 \cdot \vv^\top \left( \sum_i a_i a_i^\top \right) \vv \ge \vv^\top \left( \sum_i \tilde{a}_i \tilde{a}_i^\top \right) \vv
    \\
    \Leftrightarrow & \sum_{i=1}^n ||a_i||^2 ||g_i||^2 \cdot \left( \sum_i \vv^\top a_i a_i^\top \vv \right) \ge \vv^\top \left( \sum_i ||g_i||^2 {a}_i {a}_i^\top \right) \vv
    \\
    \Leftrightarrow & \sum_{i=1}^n ||g_i||^2 \cdot \left( \sum_i \vv^\top a_i a_i^\top \vv \right) \ge \sum_i ||g_i||^2 \vv^\top {a}_i {a}_i^\top \vv
    \\
    & \text{(we assume $||a_i|| = 1$ \clarify{(what if we don't)})}
\end{align*}
which is true. 

\end{proof}

\begin{theorem}
\begin{align}
    \|\mathbf{u}(k)-\mathbf{y}\|_{2}^{2} \leq \left( someConstant \right)^{k}\|\mathbf{u}(0)-\mathbf{y}\|_{2}^{2}
    \label{eq_6}
\end{align}
\end{theorem}

% \ref{eq_1}
% \ref{eq_2}
% \ref{eq_4}
% \ref{eq_5}
% \ref{eq_6} no
% \ref{eq_8} no

\begin{proof}

We prove it by induction. For the base case $k = 0$, (\ref{eq_6}) holds. Suppose (\ref{eq_6}) holds for $0, ..., k$, we want to show it holds for $k+1$:

We have that
\deletethis{
\begin{align*}
    \| \mathbf{y}-\mathbf{u}(k+1) \|_{2}^{2}
    = & \|\mathbf{y}-\mathbf{u}(k)-(\mathbf{u}(k+1)-\mathbf{u}(k))\|_{2}^{2} 
    \\
    \approx & \|\mathbf{y} - \mathbf{u}(k) - \eta \sum_{i=1}^n ||a_i||^2 ||g_i||^2 \left( \left( \widecheck{X} \left( \tilde{X}^\top \tilde{X} \right)^{-1} \widecheck{X}^\top \right) \odot I \right) (\vy - \vu(k)) \|_{2}^{2}
    \\
    & \text{(by Lemma \ref{lemma_1})}
    \\
    = & (\vy - \vu(k))^\top \left( I - \eta \sum_{i=1}^n ||a_i||^2 ||g_i||^2 \left( \left( \widecheck{X} \left( \tilde{X}^\top \tilde{X} \right)^{-1} \widecheck{X}^\top \right) \odot I \right) \right)^2 (\vy - \vu(k))
    \\
    \leq & \left( \lambda_{\max} \left\{  I - \eta \sum_{i=1}^n ||a_i||^2 ||g_i||^2 \left( \left( \widecheck{X} \left( \tilde{X}^\top \tilde{X} \right)^{-1} \widecheck{X}^\top \right) \odot I \right) \right\} \right)^2 \| \mathbf{y}-\mathbf{u}(k) \|_{2}^{2}
    \\
    = & \left( 1 - \eta \sum_{i=1}^n ||a_i||^2 ||g_i||^2 \cdot \lambda_{\min} \left\{ \left( \widecheck{X} \left( \tilde{X}^\top \tilde{X} \right)^{-1} \widecheck{X}^\top \right) \odot I \right\} \right)^2 \| \mathbf{y}-\mathbf{u}(k) \|_{2}^{2}
    \\
    \le & \left( 1 - \eta \sum_{i=1}^n ||a_i||^2 ||g_i||^2 \cdot \frac{1}{\lambda_{\max} \left\{ \tilde{X}^\top \tilde{X} \right\} } \right)^2 \| \mathbf{y}-\mathbf{u}(k) \|_{2}^{2}
    \\
    \le & \left( 1 - \eta \frac{1}{\lambda_{\max} \left\{ {X}^\top {X} \right\} } \right)^2 \| \mathbf{y}-\mathbf{u}(k) \|_{2}^{2}.
    \\
    & \text{(by Lemma \ref{lemma_4})}
\end{align*}
}

\addthis{
\begin{align*}
    \| \mathbf{y}-\mathbf{u}(k+1) \|_{2}^{2}
    = & \|\mathbf{y}-\mathbf{u}(k)-(\mathbf{u}(k+1)-\mathbf{u}(k))\|_{2}^{2} 
    \\
    = & \|\mathbf{y} - \mathbf{u}(k)\|_{2}^{2} + \|\mathbf{u}(k+1) - \mathbf{u}(k)\|_{2}^{2} - 2 (\mathbf{y} - \mathbf{u}(k))^\top (\mathbf{u}(k+1) - \mathbf{u}(k))
    \\
    \\
    \approx & \|\mathbf{y} - \mathbf{u}(k) - \eta \sum_{i=1}^n ||a_i||^2 ||g_i||^2 \left( \left( \widecheck{X} \left( \tilde{X}^\top \tilde{X} \right)^{-1} \widecheck{X}^\top \right) \odot I \right) (\vy - \vu(k)) \|_{2}^{2}
    \\
    & \text{(by Lemma \ref{lemma_1})}
    \\
    = & (\vy - \vu(k))^\top \left( I - \eta \sum_{i=1}^n ||a_i||^2 ||g_i||^2 \left( \left( \widecheck{X} \left( \tilde{X}^\top \tilde{X} \right)^{-1} \widecheck{X}^\top \right) \odot I \right) \right)^2 (\vy - \vu(k))
    \\
    \leq & \left( \lambda_{\max} \left\{  I - \eta \sum_{i=1}^n ||a_i||^2 ||g_i||^2 \left( \left( \widecheck{X} \left( \tilde{X}^\top \tilde{X} \right)^{-1} \widecheck{X}^\top \right) \odot I \right) \right\} \right)^2 \| \mathbf{y}-\mathbf{u}(k) \|_{2}^{2}
    \\
    = & \left( 1 - \eta \sum_{i=1}^n ||a_i||^2 ||g_i||^2 \cdot \lambda_{\min} \left\{ \left( \widecheck{X} \left( \tilde{X}^\top \tilde{X} \right)^{-1} \widecheck{X}^\top \right) \odot I \right\} \right)^2 \| \mathbf{y}-\mathbf{u}(k) \|_{2}^{2}
    \\
    \le & \left( 1 - \eta \sum_{i=1}^n ||a_i||^2 ||g_i||^2 \cdot \frac{1}{\lambda_{\max} \left\{ \tilde{X}^\top \tilde{X} \right\} } \right)^2 \| \mathbf{y}-\mathbf{u}(k) \|_{2}^{2}
    \\
    \le & \left( 1 - \eta \frac{1}{\lambda_{\max} \left\{ {X}^\top {X} \right\} } \right)^2 \| \mathbf{y}-\mathbf{u}(k) \|_{2}^{2}.
    \\
    & \text{(by Lemma \ref{lemma_4})}
\end{align*}
}

\end{proof}
